# Supplementary material for: Spin accumulation without spin current
Source: arXiv:2112.11043 source file (2022-05-12)
Supplement: Supplementary file 1 [file suppl.pdf]

# Supplemental Material for "Spin accumulation without spin current"


Atsuo Shitade[1] and Gen Tatara[2]

[1]Institute for Molecular Science, Aichi 444-8585, Japan

[2]RIKEN Center for Emergent Matter Science (CEMS) and RIKEN Cluster for Pioneering Research (CPR), 2-1 Hirosawa, Wako, Saitama 351-0198, Japan



(Dated: May 7, 2022)


## BLOCH FORMULAS

### Conventional spin current

First, we write down the Bloch formula for the spin (Hall) conductivity of the conventional spin current [1]. The spin-current–charge-current correlation function that characterizes $\langle \Delta \hat{J}_{sa}{}^i \rangle(\Omega, \boldsymbol{Q}) = \chi^{\mathrm{R}}_{\hat{J}_{sa}{}^i \hat{j}^j}(\Omega, \boldsymbol{Q}) A_j(\Omega, \boldsymbol{Q})$ is expressed as

$$\begin{aligned}\chi^{\mathrm{R}}_{\hat{J}_{sa}{}^i \hat{j}^j}(\Omega, \boldsymbol{Q}) =& -q \sum_{nm} \int \frac{d^d k}{(2\pi)^d} \langle u_n(\boldsymbol{k}_-)|\hat{J}_{sa}{}^i(\boldsymbol{k};\boldsymbol{Q})|u_m(\boldsymbol{k}_+)\rangle \langle u_m(\boldsymbol{k}_+)|\hat{v}^j(\boldsymbol{k};\boldsymbol{Q})|u_n(\boldsymbol{k}_-)\rangle \frac{f(\epsilon_n(\boldsymbol{k}_-)) - f(\epsilon_m(\boldsymbol{k}_+))}{\hbar\Omega + \epsilon_n(\boldsymbol{k}_-) - \epsilon_m(\boldsymbol{k}_+) + i\eta} \\ =& \chi^{\mathrm{R}}_{\hat{J}_{sa}{}^i \hat{j}^j}(0, \boldsymbol{Q}) + (i\Omega)\sigma^{\mathrm{R}}_{\hat{J}_{sa}{}^i \hat{j}^j}(\Omega, \boldsymbol{Q}),\end{aligned} \tag{1}$$

where $q$ is the electron charge, $d$ is the spatial dimension, $\eta \to +0$ is the convergence factor, $\hat{J}_{sa}{}^i(\boldsymbol{k};\boldsymbol{Q}) = [\hat{J}_{sa}{}^i(\boldsymbol{k}_+) + \hat{J}_{sa}{}^i(\boldsymbol{k}_-)]/2$ with $\boldsymbol{k}_\pm = \boldsymbol{k} \pm \boldsymbol{Q}/2$, and $f(\epsilon) = [e^{(\epsilon-\mu)/T} + 1]^{-1}$ is the Fermi distribution function. The spin (Hall) conductivity is obtained from

$$\begin{aligned}\sigma^{\mathrm{R}}_{\hat{J}_{sa}{}^i \hat{j}^j}(\Omega, \boldsymbol{Q}) =& [\chi^{\mathrm{R}}_{\hat{J}_{sa}{}^i \hat{j}^j}(\Omega, \boldsymbol{Q}) - \chi_{\hat{J}_{sa}{}^i \hat{j}^j}(0, \boldsymbol{Q})]/(i\Omega) \\ =& -i\hbar q \sum_{nm} \int \frac{d^d k}{(2\pi)^d} \langle u_n(\boldsymbol{k}_-)|\hat{J}_{sa}{}^i(\boldsymbol{k};\boldsymbol{Q})|u_m(\boldsymbol{k}_+)\rangle \langle u_m(\boldsymbol{k}_+)|\hat{v}^j(\boldsymbol{k};\boldsymbol{Q})|u_n(\boldsymbol{k}_-)\rangle \\ & \times \frac{f(\epsilon_n(\boldsymbol{k}_-)) - f(\epsilon_m(\boldsymbol{k}_+))}{[\hbar\Omega + \epsilon_n(\boldsymbol{k}_-) - \epsilon_m(\boldsymbol{k}_+) + i\eta][\epsilon_n(\boldsymbol{k}_-) - \epsilon_m(\boldsymbol{k}_+)]},\end{aligned} \tag{2}$$

in the limits of $\Omega \to 0$ and $\boldsymbol{Q} \to 0$. The intraband $n = m$ and interband $n \neq m$ contributions are

$$\begin{aligned}\sigma^{\mathrm{R(I)}}_{\hat{J}_{sa}{}^i \hat{j}^j}(0, \boldsymbol{Q}) =& -i\hbar q \sum_{n} \int \frac{d^d k}{(2\pi)^d} \langle u_n(\boldsymbol{k}_-)|\hat{J}_{sa}{}^i(\boldsymbol{k};\boldsymbol{Q})|u_n(\boldsymbol{k}_+)\rangle \langle u_n(\boldsymbol{k}_+)|\hat{v}^j(\boldsymbol{k};\boldsymbol{Q})|u_n(\boldsymbol{k}_-)\rangle \\ & \times \frac{f(\epsilon_n(\boldsymbol{k}_-)) - f(\epsilon_n(\boldsymbol{k}_+))}{[\epsilon_n(\boldsymbol{k}_-) - \epsilon_n(\boldsymbol{k}_+) + i\eta][\epsilon_n(\boldsymbol{k}_-) - \epsilon_n(\boldsymbol{k}_+)]} \\ =& -\frac{\hbar q}{\eta} \sum_{n} \int \frac{d^d k}{(2\pi)^d} \langle u_n|\hat{J}_{sa}{}^i|u_n\rangle \langle u_n|\hat{v}^j|u_n\rangle f'(\epsilon_n),\end{aligned} \tag{3a}$$

$$\begin{aligned}\sigma^{\mathrm{R(II)}}_{\hat{J}_{sa}{}^i \hat{j}^j}(0, \boldsymbol{Q}) =& -i\hbar q \sum_{n \neq m} \int \frac{d^d k}{(2\pi)^d} \langle u_n(\boldsymbol{k}_-)|\hat{J}_{sa}{}^i(\boldsymbol{k};\boldsymbol{Q})|u_m(\boldsymbol{k}_+)\rangle \langle u_m(\boldsymbol{k}_+)|\hat{v}^j(\boldsymbol{k};\boldsymbol{Q})|u_n(\boldsymbol{k}_-)\rangle \frac{f(\epsilon_n(\boldsymbol{k}_-)) - f(\epsilon_m(\boldsymbol{k}_+))}{[\epsilon_n(\boldsymbol{k}_-) - \epsilon_m(\boldsymbol{k}_+)]^2} \\ =& -i\hbar q \sum_{n \neq m} \int \frac{d^d k}{(2\pi)^d} \langle u_n|\hat{J}_{sa}{}^i|u_m\rangle \langle u_m|\hat{v}^j|u_n\rangle \frac{f(\epsilon_n) - f(\epsilon_m)}{(\epsilon_n - \epsilon_m)^2} \\ =& -i\hbar q \sum_{n \neq m} \int \frac{d^d k}{(2\pi)^d} \frac{\langle u_n|\hat{J}_{sa}{}^i|u_m\rangle \langle u_m|\hat{v}^j|u_n\rangle - \mathrm{c.c.}}{(\epsilon_n - \epsilon_m)^2} f(\epsilon_n) \\ =& -\frac{q}{\hbar} \sum_{n} \int \frac{d^d k}{(2\pi)^d} b_{sna}{}^{ij} f(\epsilon_n).\end{aligned} \tag{3b}$$

The argument of $\boldsymbol{k}$ is omitted for simplicity. $b_{sna}{}^{ij}$ is defined as

$$b_{sna}{}^{ij} = i \sum_{m(\neq n)} \frac{\langle u_n|\hbar\hat{J}_{sa}{}^i|u_m\rangle \langle u_m|\hbar\hat{v}^j|u_n\rangle - \mathrm{c.c.}}{(\epsilon_n - \epsilon_m)^2}, \tag{4}$$

which is reduced to the Berry curvature when $\hat{s}_a$ is replaced by 1. We neglect Eq. (3a) that is proportional to the phenomenological relaxation time $\hbar/\eta$. Thus, the intrinsic spin (Hall) conductivity of the conventional spin current is expressed as

$$\sigma_{sa}{}^{ij(\mathrm{II})} = -\frac{q}{\hbar}\sum_n \int \frac{d^dk}{(2\pi)^d} b_{sna}{}^{ij} f(\epsilon_n). \tag{5}$$

### Conserved spin current

Second, we derive the Bloch formula for the spin (Hall) conductivity of the conserved spin current proposed in Refs. [2, 3]. The spin torque operator is defined as $\hat{\tau}_a(\boldsymbol{k}) = [\hat{s}_a, \hat{\mathcal{H}}(\boldsymbol{k})]/i\hbar$. The spin-torque–charge-current correlation function that characterizes $\langle \Delta\hat{\tau}_a\rangle(\Omega,\boldsymbol{Q}) = \chi^{\mathrm{R}}_{\hat{\tau}_a \hat{j}^j}(\Omega,\boldsymbol{Q})A_j(\Omega,\boldsymbol{Q})$ is expressed as

$$\begin{aligned}\chi^{\mathrm{R}}_{\hat{\tau}_a \hat{j}^j}(\Omega,\boldsymbol{Q}) =& -q\sum_{nm}\int \frac{d^dk}{(2\pi)^d}\langle u_n(\boldsymbol{k}_-)|\hat{\tau}_a(\boldsymbol{k};\boldsymbol{Q})|u_m(\boldsymbol{k}_+)\rangle\langle u_m(\boldsymbol{k}_+)|\hat{v}^j(\boldsymbol{k};\boldsymbol{Q})|u_n(\boldsymbol{k}_-)\rangle \frac{f(\epsilon_n(\boldsymbol{k}_-)) - f(\epsilon_m(\boldsymbol{k}_+))}{\hbar\Omega + \epsilon_n(\boldsymbol{k}_-) - \epsilon_m(\boldsymbol{k}_+) + i\eta} \\ =& \chi^{\mathrm{R}}_{\hat{\tau}_a \hat{j}^j}(0,\boldsymbol{Q}) + (i\Omega)\sigma^{\mathrm{R}}_{\hat{\tau}_a \hat{j}^j}(\Omega,\boldsymbol{Q}).\end{aligned} \tag{6}$$

Here, we expand the response to the electric field,

$$\begin{aligned}\sigma^{\mathrm{R}}_{\hat{\tau}_a \hat{j}^j}(\Omega,\boldsymbol{Q}) =& [\chi^{\mathrm{R}}_{\hat{\tau}_a \hat{j}^j}(\Omega,\boldsymbol{Q}) - \chi_{\hat{\tau}_a \hat{j}^j}(0,\boldsymbol{Q})]/(i\Omega) \\ =& -i\hbar q \sum_{nm}\int \frac{d^dk}{(2\pi)^d}\langle u_n(\boldsymbol{k}_-)|\hat{\tau}_a(\boldsymbol{k};\boldsymbol{Q})|u_m(\boldsymbol{k}_+)\rangle\langle u_m(\boldsymbol{k}_+)|\hat{v}^j(\boldsymbol{k};\boldsymbol{Q})|u_n(\boldsymbol{k}_-)\rangle \\ & \times \frac{f(\epsilon_n(\boldsymbol{k}_-)) - f(\epsilon_m(\boldsymbol{k}_+))}{[\hbar\Omega + \epsilon_n(\boldsymbol{k}_-) - \epsilon_m(\boldsymbol{k}_+) + i\eta][\epsilon_n(\boldsymbol{k}_-) - \epsilon_m(\boldsymbol{k}_+)]},\end{aligned} \tag{7}$$

up to the first order with respect to $\boldsymbol{Q}$ at $\Omega \to 0$. The intraband $n = m$ and interband $n \neq m$ contributions are

$$\begin{aligned}\sigma^{\mathrm{R(I)}}_{\hat{\tau}_a \hat{j}^j}(0,\boldsymbol{Q}) =& -i\hbar q\sum_n\int \frac{d^dk}{(2\pi)^d}\langle u_n(\boldsymbol{k}_-)|\hat{\tau}_a(\boldsymbol{k};\boldsymbol{Q})|u_n(\boldsymbol{k}_+)\rangle\langle u_n(\boldsymbol{k}_+)|\hat{v}^j(\boldsymbol{k};\boldsymbol{Q})|u_n(\boldsymbol{k}_-)\rangle \\ & \times \frac{f(\epsilon_n(\boldsymbol{k}_-)) - f(\epsilon_n(\boldsymbol{k}_+))}{[\epsilon_n(\boldsymbol{k}_-) - \epsilon_n(\boldsymbol{k}_+) + i\eta][\epsilon_n(\boldsymbol{k}_-) - \epsilon_n(\boldsymbol{k}_+)]} \\ =& -\frac{\hbar q}{\eta}\sum_n\int\frac{d^dk}{(2\pi)^d}\langle u_n|\hat{\tau}_a|u_n\rangle\langle u_n|\hat{v}^j|u_n\rangle f'(\epsilon_n) + \frac{\hbar q Q_i}{2\eta}\sum_n\int\frac{d^dk}{(2\pi)^d} \\ & \times [(\langle\partial_{k_i}u_n|\hat{\tau}_a|u_n\rangle - \langle u_n|\hat{\tau}_a|\partial_{k_i}u_n\rangle)\langle u_n|\hat{v}^j|u_n\rangle - \langle u_n|\hat{\tau}_a|u_n\rangle(\langle\partial_{k_i}u_n|\hat{v}^j|u_n\rangle - \langle u_n|\hat{v}^j|\partial_{k_i}u_n\rangle)]f'(\epsilon_n) \\ & + \frac{i\hbar q Q_i}{\eta^2}\sum_n\int\frac{d^dk}{(2\pi)^d}\langle u_n|\hat{\tau}_a|u_n\rangle\langle u_n|\hat{v}^j|u_n\rangle\partial_{k_i}\epsilon_n f'(\epsilon_n) \\ =& -\frac{\hbar q}{\eta}\sum_n\int\frac{d^dk}{(2\pi)^d}\langle u_n|\hat{\tau}_a|u_n\rangle\langle u_n|\hat{v}^j|u_n\rangle f'(\epsilon_n) \\ & + \frac{\hbar q Q_i}{2\eta}\sum_n\int\frac{d^dk}{(2\pi)^d}[(\langle\partial_{k_i}u_n|\hat{Q}_n\hat{\tau}_a|u_n\rangle - \mathrm{c.c.})\langle u_n|\hat{v}^j|u_n\rangle - \langle u_n|\hat{\tau}_a|u_n\rangle(\langle\partial_{k_i}u_n|\hat{Q}_n\hat{v}^j|u_n\rangle - \mathrm{c.c.})]f'(\epsilon_n) \\ & + \frac{i\hbar q Q_i}{\eta^2}\sum_n\int\frac{d^dk}{(2\pi)^d}\langle u_n|\hat{\tau}_a|u_n\rangle\langle u_n|\hat{v}^j|u_n\rangle\partial_{k_i}\epsilon_n f'(\epsilon_n) \\ =& \frac{\hbar q Q_i}{2\eta}\sum_n\int\frac{d^dk}{(2\pi)^d}(\langle\partial_{k_i}u_n|\hat{Q}_n\hat{\tau}_a|u_n\rangle - \mathrm{c.c.})\langle u_n|\hat{v}^j|u_n\rangle f'(\epsilon_n),\end{aligned} \tag{8a}$$

$$\begin{aligned}\sigma^{\mathrm{R(II)}}_{\hat{\tau}_a \hat{j}^j}(0,\boldsymbol{Q}) =& -i\hbar q\sum_{n\neq m}\int\frac{d^dk}{(2\pi)^d}\langle u_n(\boldsymbol{k}_-)|\hat{\tau}_a(\boldsymbol{k};\boldsymbol{Q})|u_m(\boldsymbol{k}_+)\rangle\langle u_m(\boldsymbol{k}_+)|\hat{v}^j(\boldsymbol{k};\boldsymbol{Q})|u_n(\boldsymbol{k}_-)\rangle\frac{f(\epsilon_n(\boldsymbol{k}_-)) - f(\epsilon_m(\boldsymbol{k}_+))}{[\epsilon_n(\boldsymbol{k}_-) - \epsilon_m(\boldsymbol{k}_+)]^2} \\ =& -i\hbar q\sum_{n\neq m}\int\frac{d^dk}{(2\pi)^d}\langle u_n|\hat{\tau}_a|u_m\rangle\langle u_m|\hat{v}^j|u_n\rangle\frac{f(\epsilon_n) - f(\epsilon_m)}{(\epsilon_n - \epsilon_m)^2} + \frac{i\hbar q Q_i}{2}\sum_{n\neq m}\int\frac{d^dk}{(2\pi)^d}\end{aligned}$$

$$
\begin{aligned}
&\times \Bigg\{ [(\langle \partial_{k_i} u_n | \hat{\tau}_a | u_m\rangle - \langle u_n | \hat{\tau}_a | \partial_{k_i} u_m\rangle)\langle u_m | \hat{v}^j | u_n\rangle + \langle u_n | \hat{\tau}_a | u_m\rangle(\langle u_m | \hat{v}^j | \partial_{k_i} u_n\rangle - \langle \partial_{k_i} u_m | \hat{v}^j | u_n\rangle)] \\
&\times \frac{f(\epsilon_n) - f(\epsilon_m)}{(\epsilon_n - \epsilon_m)^2} + \langle u_n | \hat{\tau}_a | u_m\rangle\langle u_m | \hat{v}^j | u_n\rangle \left[\frac{\partial_{k_i}\epsilon_n f'(\epsilon_n) + \partial_{k_i}\epsilon_m f'(\epsilon_m)}{(\epsilon_n - \epsilon_m)^2} - 2\frac{\partial_{k_i}(\epsilon_n + \epsilon_m)}{\epsilon_n - \epsilon_m}\frac{f(\epsilon_n) - f(\epsilon_m)}{(\epsilon_n - \epsilon_m)^2}\right]\Bigg\} \\
=& - i\hbar q \sum_{n\neq m}\int \frac{d^dk}{(2\pi)^d}\frac{\langle u_n | \hat{\tau}_a | u_m\rangle\langle u_m | \hat{v}^j | u_n\rangle - \text{c.c.}}{(\epsilon_n - \epsilon_m)^2} f(\epsilon_n) + \frac{i\hbar q Q_i}{2}\sum_{n\neq m}\int\frac{d^dk}{(2\pi)^d} \\
&\times \Bigg\{ \frac{(\langle \partial_{k_i} u_n | \hat{\tau}_a | u_m\rangle - \langle u_n | \hat{\tau}_a | \partial_{k_i} u_m\rangle)\langle u_m | \hat{v}^j | u_n\rangle + \text{c.c.} + \langle u_n | \hat{\tau}_a | u_m\rangle(\langle u_m | \hat{v}^j | \partial_{k_i} u_n\rangle - \langle \partial_{k_i} u_m | \hat{v}^j | u_n\rangle) + \text{c.c.}}{(\epsilon_n - \epsilon_m)^2} \\
&\times f(\epsilon_n) + \frac{\langle u_n | \hat{\tau}_a | u_m\rangle\langle u_m | \hat{v}^j | u_n\rangle + \text{c.c.}}{(\epsilon_n - \epsilon_m)^2}\left[\partial_{k_i}\epsilon_n f'(\epsilon_n) - 2\frac{\partial_{k_i}(\epsilon_n + \epsilon_m)}{\epsilon_n - \epsilon_m} f(\epsilon_n)\right]\Bigg\} \\
=& \frac{q}{\hbar}\sum_{n\neq m}\int\frac{d^dk}{(2\pi)^d}(\langle u_n | \hat{s}_a | u_m\rangle\langle u_m | \partial_{k_j} u_n\rangle + \text{c.c.}) f(\epsilon_n) \\
&- \frac{qQ_i}{2\hbar}\sum_{n\neq m}\int\frac{d^dk}{(2\pi)^d}(\langle u_n | \hat{s}_a | u_m\rangle\langle u_m | \partial_{k_j} u_n\rangle - \text{c.c.})\partial_{k_i}\epsilon_n f'(\epsilon_n) + (\text{Fermi-sea terms}) \\
=& \frac{q}{\hbar}\sum_{n}\int\frac{d^dk}{(2\pi)^d}(\langle u_n | \hat{s}_a\hat{Q}_n | \partial_{k_j} u_n\rangle + \text{c.c.}) f(\epsilon_n) \\
&- \frac{qQ_i}{2\hbar}\sum_{n}\int\frac{d^dk}{(2\pi)^d}(\langle u_n | \hat{s}_a\hat{Q}_n | \partial_{k_j} u_n\rangle - \text{c.c.})\partial_{k_i}\epsilon_n f'(\epsilon_n) + (\text{Fermi-sea terms}) \\
=& \frac{q}{\hbar}\sum_{n}\int\frac{d^dk}{(2\pi)^d}\partial_{k_j} s_{na} f(\epsilon_n) + \frac{q(iQ_i)}{\hbar}\sum_n\int\frac{d^dk}{(2\pi)^d}[{s_{na}}^j\partial_{k_i}\epsilon_n f'(\epsilon_n) + (\epsilon^{ijk}b_{nak} - {b_{sna}}^{ij}) f(\epsilon_n)].
\end{aligned} \tag{8b}
$$

Here, $\hat{Q}_n = 1 - |u_n\rangle\langle u_n|$ is the antiprojection operator, and we have used

$$\langle u_m | \hbar\hat{v}^j | u_n\rangle = \partial_{k_j}\epsilon_n\delta_{mn} + (\epsilon_n - \epsilon_m)\langle u_m | \partial_{k_j} u_n\rangle, \tag{9a}$$

$$\langle u_m | \hat{\tau}_a | u_n\rangle = \frac{1}{i\hbar}(\epsilon_n - \epsilon_m)\langle u_m | \hat{s}_a | u_n\rangle. \tag{9b}$$

In particular, $\langle u_n | \hat{\tau}_a | u_n\rangle = 0$. We have also introduced $s_{na} = \langle u_n | \hat{s}_a | u_n\rangle$, the magnetic moment $m_{nk}$ [4–6], spin magnetic quadrupole moment ${s_{na}}^i$ [7, 8], and spin Berry curvature $b_{nka}$ as

$$\epsilon^{ijk} m_{nk} = -\frac{i}{2}[\langle \partial_{k_i} u_n | (\epsilon_n - \hat{\mathcal{H}}) | \partial_{k_j} u_n\rangle - \text{c.c.}], \tag{10a}$$

$${s_{na}}^i = -\frac{i}{2}(\langle \partial_{k_i} u_n | \hat{Q}_n \hat{s}_a | u_n\rangle - \text{c.c.}), \tag{10b}$$

$$
\begin{aligned}
\epsilon^{ijk} b_{nak} =& \frac{i}{2}[\langle \partial_{k_i} u_n | \hat{Q}_n (s_{na} + \hat{s}_a)\hat{Q}_n | \partial_{k_j} u_n\rangle - \text{c.c.}] \\
&- \frac{i}{2}\sum_{m(\neq n)}\frac{\langle u_n | \hat{s}_a | u_m\rangle[\langle u_m | (\partial_{k_i}\epsilon_n + \hbar\hat{v}^i)\hat{Q}_n | \partial_{k_j} u_n\rangle - (i \leftrightarrow j)] - \text{c.c.}}{\epsilon_n - \epsilon_m}.
\end{aligned} \tag{10c}
$$

Concerning the Fermi-sea terms in Eq. (8b), we insert $|u_l\rangle\langle u_l|$ to obtain

$$
\begin{aligned}
&\frac{\hbar^2}{2}\sum_{m(\neq n)}\frac{(\langle \partial_{k_i} u_n | \hat{\tau}_a | u_m\rangle - \langle u_n | \hat{\tau}_a | \partial_{k_i} u_m\rangle)\langle u_m | \hat{v}^j | u_n\rangle + \text{c.c.} + \langle u_n | \hat{\tau}_a | u_m\rangle(\langle u_m | \hat{v}^j | \partial_{k_i} u_n\rangle - \langle \partial_{k_i} u_m | \hat{v}^j | u_n\rangle) + \text{c.c.}}{(\epsilon_n - \epsilon_m)^2} \\
&- \hbar^2\sum_{m(\neq n)}\frac{\langle u_n | \hat{\tau}_a | u_m\rangle\partial_{k_i}(\epsilon_n + \epsilon_m)\langle u_m | \hat{v}^j | u_n\rangle + \text{c.c.}}{(\epsilon_n - \epsilon_m)^3} \\
=& \frac{\hbar^2}{2}\sum_{l\neq m(\neq n)}\Bigg[\frac{\langle \partial_{k_i} u_n | u_l\rangle\langle u_l | \hat{\tau}_a | u_m\rangle\langle u_m | \hat{v}^j | u_n\rangle + \text{c.c.}}{(\epsilon_n - \epsilon_m)^2} - \frac{\langle u_n | \hat{\tau}_a | u_l\rangle\langle u_l | \partial_{k_i} u_m\rangle\langle u_m | \hat{v}^j | u_n\rangle + \text{c.c.}}{(\epsilon_n - \epsilon_m)^2} \\
&+ \frac{\langle u_n | \hat{\tau}_a | u_m\rangle\langle u_m | \hat{v}^j | u_l\rangle\langle u_l | \partial_{k_i} u_n\rangle + \text{c.c.}}{(\epsilon_n - \epsilon_m)^2} - \frac{\langle u_n | \hat{\tau}_a | u_m\rangle\langle \partial_{k_i} u_m | u_l\rangle\langle u_l | \hat{v}^j | u_n\rangle + \text{c.c.}}{(\epsilon_n - \epsilon_m)^2}\Bigg]
\end{aligned}
$$

$$
\begin{aligned}
&+\frac{\hbar^2}{2}\sum_{m(\neq n)}\Bigg[\frac{\langle\partial_{k_i}u_n|u_n\rangle\langle u_n|\hat{\tau}_a|u_m\rangle\langle u_m|\hat{v}^j|u_n\rangle+\text{c.c.}}{(\epsilon_n-\epsilon_m)^2}-\frac{\langle u_n|\hat{\tau}_a|u_n\rangle\langle u_n|\partial_{k_i}u_m\rangle\langle u_m|\hat{v}^j|u_n\rangle+\text{c.c.}}{(\epsilon_n-\epsilon_m)^2}\\
&+\frac{\langle u_n|\hat{\tau}_a|u_m\rangle\langle u_m|\hat{v}^j|u_n\rangle\langle u_n|\partial_{k_i}u_n\rangle+\text{c.c.}}{(\epsilon_n-\epsilon_m)^2}-\frac{\langle u_n|\hat{\tau}_a|u_m\rangle\langle\partial_{k_i}u_m|u_n\rangle\langle u_n|\hat{v}^j|u_n\rangle+\text{c.c.}}{(\epsilon_n-\epsilon_m)^2}\\
&+\frac{\langle\partial_{k_i}u_n|u_m\rangle\langle u_m|\hat{\tau}_a|u_m\rangle\langle u_m|\hat{v}^j|u_n\rangle+\text{c.c.}}{(\epsilon_n-\epsilon_m)^2}-\frac{\langle u_n|\hat{\tau}_a|u_m\rangle\langle u_m|\partial_{k_i}u_m\rangle\langle u_m|\hat{v}^j|u_n\rangle+\text{c.c.}}{(\epsilon_n-\epsilon_m)^2}\\
&+\frac{\langle u_n|\hat{\tau}_a|u_m\rangle\langle u_m|\hat{v}^j|u_m\rangle\langle u_m|\partial_{k_i}u_n\rangle+\text{c.c.}}{(\epsilon_n-\epsilon_m)^2}-\frac{\langle u_n|\hat{\tau}_a|u_m\rangle\langle\partial_{k_i}u_m|u_m\rangle\langle u_m|\hat{v}^j|u_n\rangle+\text{c.c.}}{(\epsilon_n-\epsilon_m)^2}\\
&-2\frac{\langle u_n|\hat{\tau}_a|u_m\rangle\partial_{k_i}(\epsilon_n+\epsilon_m)\langle u_m|\hat{v}^j|u_n\rangle+\text{c.c.}}{(\epsilon_n-\epsilon_m)^3}\Bigg]\\
=&\frac{\hbar^3}{2}\sum_{l\neq m(\neq n)}\Bigg[\frac{\langle u_n|\hat{v}^i|u_l\rangle\langle u_l|\hat{\tau}_a|u_m\rangle\langle u_m|\hat{v}^j|u_n\rangle+\text{c.c.}}{(\epsilon_n-\epsilon_m)^2(\epsilon_n-\epsilon_l)}-\frac{\langle u_n|\hat{\tau}_a|u_l\rangle\langle u_l|\hat{v}^i|u_m\rangle\langle u_m|\hat{v}^j|u_n\rangle+\text{c.c.}}{(\epsilon_n-\epsilon_m)^2(\epsilon_m-\epsilon_l)}\\
&+\frac{\langle u_n|\hat{\tau}_a|u_m\rangle\langle u_m|\hat{v}^j|u_l\rangle\langle u_l|\hat{v}^i|u_n\rangle+\text{c.c.}}{(\epsilon_n-\epsilon_m)^2(\epsilon_n-\epsilon_l)}-\frac{\langle u_n|\hat{\tau}_a|u_m\rangle\langle u_m|\hat{v}^i|u_l\rangle\langle u_l|\hat{v}^j|u_n\rangle+\text{c.c.}}{(\epsilon_n-\epsilon_m)^2(\epsilon_m-\epsilon_l)}\Bigg]\\
&+\frac{\hbar^3}{2}\sum_{m(\neq n)}\Bigg[\frac{\langle u_n|\hat{\tau}_a|u_n\rangle\langle u_n|\hat{v}^i|u_m\rangle\langle u_m|\hat{v}^j|u_n\rangle+\text{c.c.}}{(\epsilon_n-\epsilon_m)^3}+\frac{\langle u_n|\hat{\tau}_a|u_m\rangle\langle u_m|\hat{v}^i|u_n\rangle\langle u_n|\hat{v}^j|u_n\rangle+\text{c.c.}}{(\epsilon_n-\epsilon_m)^3}\\
&+\frac{\langle u_n|\hat{v}^i|u_m\rangle\langle u_m|\hat{\tau}_a|u_m\rangle\langle u_m|\hat{v}^j|u_n\rangle+\text{c.c.}}{(\epsilon_n-\epsilon_m)^3}+\frac{\langle u_n|\hat{\tau}_a|u_m\rangle\langle u_m|\hat{v}^j|u_m\rangle\langle u_m|\hat{v}^i|u_n\rangle+\text{c.c.}}{(\epsilon_n-\epsilon_m)^3}\\
&-2\frac{\langle u_n|\hat{\tau}_a|u_m\rangle(\langle u_n|\hat{v}^i|u_n\rangle+\langle u_m|\hat{v}^i|u_m\rangle)\langle u_m|\hat{v}^j|u_n\rangle+\text{c.c.}}{(\epsilon_n-\epsilon_m)^3}\Bigg]\\
=&\frac{\hbar^3}{2}\sum_{l\neq m(\neq n)}\Bigg\{\frac{\langle u_n|\hat{v}^i|u_m\rangle\langle u_m|\hat{\tau}_a|u_l\rangle\langle u_l|\hat{v}^j|u_n\rangle+\text{c.c.}-\langle u_n|\hat{\tau}_a|u_m\rangle\langle u_m|\hat{v}^i|u_l\rangle\langle u_l|\hat{v}^j|u_n\rangle+\text{c.c.}}{(\epsilon_n-\epsilon_m)(\epsilon_n-\epsilon_l)^2}\\
&-\frac{\langle u_n|\hat{\tau}_a|u_m\rangle[\langle u_m|\hat{v}^i|u_l\rangle\langle u_l|\hat{v}^j|u_n\rangle-(i\leftrightarrow j)]+\text{c.c.}}{(\epsilon_n-\epsilon_m)^2(\epsilon_n-\epsilon_l)}\Bigg\}\\
&+\frac{\hbar^3}{2}\sum_{m(\neq n)}\Bigg[\frac{\langle u_n|\hat{v}^i|u_m\rangle(\langle u_n|\hat{\tau}_a|u_n\rangle+\langle u_m|\hat{\tau}_a|u_m\rangle)\langle u_m|\hat{v}^j|u_n\rangle+\text{c.c.}-\langle u_n|\hat{\tau}_a|u_m\rangle(\langle u_n|\hat{v}^i|u_n\rangle+\langle u_m|\hat{v}^i|u_m\rangle)\langle u_m|\hat{v}^j|u_n\rangle+\text{c.c.}}{(\epsilon_n-\epsilon_m)^3}\\
&-\frac{\langle u_n|\hat{\tau}_a|u_m\rangle[(\langle u_n|\hat{v}^i|u_n\rangle+\langle u_m|\hat{v}^i|u_m\rangle)\langle u_m|\hat{v}^j|u_n\rangle-(i\leftrightarrow j)]+\text{c.c.}}{(\epsilon_n-\epsilon_m)^3}\Bigg]\\
=&\frac{\hbar^3}{2}\sum_{l,m(\neq n)}\Bigg\{\frac{\langle u_n|\hat{v}^i|u_m\rangle\langle u_m|((\langle u_n|\hat{\tau}_a|u_n\rangle+\hat{\tau}_a)|u_l\rangle\langle u_l|\hat{v}^j|u_n\rangle+\text{c.c.}-\langle u_n|\hat{\tau}_a|u_m\rangle\langle u_m|((\langle u_n|\hat{v}^i|u_n\rangle+\hat{v}^i)|u_l\rangle\langle u_l|\hat{v}^j|u_n\rangle+\text{c.c.}}{(\epsilon_n-\epsilon_m)(\epsilon_n-\epsilon_l)^2}\\
&-\frac{\langle u_n|\hat{\tau}_a|u_m\rangle[\langle u_m|((\langle u_n|\hat{v}^i|u_n\rangle+\hat{v}^i)|u_l\rangle\langle u_l|\hat{v}^j|u_n\rangle-(i\leftrightarrow j)]+\text{c.c.}}{(\epsilon_n-\epsilon_m)^2(\epsilon_n-\epsilon_l)}\Bigg\}\\
=&\frac{i}{2}\sum_{l,m(\neq n)}\Bigg\{\frac{(\epsilon_m-\epsilon_l)\langle\partial_{k_i}u_n|u_m\rangle\langle u_m|\hat{s}_a|u_l\rangle\langle u_l|\partial_{k_j}u_n\rangle-\text{c.c.}-\langle u_n|\hat{s}_a|u_m\rangle\langle u_m|(\partial_{k_i}\epsilon_n+\hbar\hat{v}^i)|u_l\rangle\langle u_l|\partial_{k_j}u_n\rangle-\text{c.c.}}{\epsilon_n-\epsilon_l}\\
&-\frac{\langle u_n|\hat{s}_a|u_m\rangle[\langle u_m|(\partial_{k_i}\epsilon_n+\hbar\hat{v}^i)|u_l\rangle\langle u_l|\partial_{k_j}u_n\rangle-(i\leftrightarrow j)]-\text{c.c.}}{\epsilon_n-\epsilon_m}\Bigg\}\\
=&\frac{i}{2}\sum_{m(\neq n)}\Bigg\{\langle\partial_{k_i}u_n|u_m\rangle\langle u_m|\hat{s}_a\hat{Q}_n|\partial_{k_j}u_n\rangle-\text{c.c.}-\frac{\langle u_n|\hat{s}_a|u_m\rangle[\langle u_m|(\partial_{k_i}\epsilon_n+\hbar\hat{v}^i)\hat{Q}_n|\partial_{k_j}u_n\rangle-(i\leftrightarrow j)]-\text{c.c.}}{\epsilon_n-\epsilon_m}\\
&-\frac{\langle u_n|[\hbar\hat{v}^i\hat{Q}_n\hat{s}_a+\hat{s}_a\hat{Q}_n(\partial_{k_i}\epsilon_n+\hbar\hat{v}^i)]|u_m\rangle\langle u_m|\partial_{k_j}u_n\rangle-\text{c.c.}}{\epsilon_n-\epsilon_m}\Bigg\}\\
=&\frac{i}{2}\sum_{m(\neq n)}\Bigg\{\langle\partial_{k_i}u_n|u_m\rangle\langle u_m|(s_{na}+\hat{s}_a\hat{Q}_n)|\partial_{k_j}u_n\rangle-\text{c.c.}-\frac{\langle u_n|\hat{s}_a|u_m\rangle[\langle u_m|(\partial_{k_i}\epsilon_n+\hbar\hat{v}^i)\hat{Q}_n|\partial_{k_j}u_n\rangle-(i\leftrightarrow j)]-\text{c.c.}}{\epsilon_n-\epsilon_m}
\end{aligned}
$$

$$-\frac{\langle u_n|(\hbar\hat{v}^i\hat{s}_a+\hat{s}_a\hbar\hat{v}^i)|u_m\rangle\langle u_m|\partial_{k_j}u_n\rangle-\text{c.c.}}{\epsilon_n-\epsilon_m}\Bigg\}$$
$$=\epsilon^{ijk}b_{nak}-{b_{sna}}^{ij}. \tag{11}$$

Again, we neglect Eq. (8a) that is proportional to $\hbar/\eta$. The first term in Eq. (8b) is the spin torque owing to the Edelstein effect, and the second term corresponds to the spin torque dipole density. Thus, we arrive at the intrinsic spin (Hall) conductivity of the conserved spin current,

$$\tilde{\sigma}_{sa}{}^{ij(\mathrm{II})}=-\frac{q}{\hbar}\sum_n\int\frac{d^dk}{(2\pi)^d}[{s_{na}}^j\partial_{k_i}\epsilon_nf'(\epsilon_n)+\epsilon^{ijk}b_{nak}f(\epsilon_n)]. \tag{12}$$

### spin-orbit magnetic susceptibility

We also write down the Bloch formula for the spin-orbit magnetic susceptibility [9]. The spin–charge-current correlation function that characterizes $\langle\Delta\hat{s}_a\rangle(\Omega,\boldsymbol{Q})=\chi^{\mathrm{R}}_{\hat{s}_a\hat{j}^j}(\Omega,\boldsymbol{Q})A_j(\Omega,\boldsymbol{Q})$ is expressed as

$$\begin{aligned}\chi^{\mathrm{R}}_{\hat{s}_a\hat{j}^j}(\Omega,\boldsymbol{Q})=&-q\sum_{nm}\int\frac{d^dk}{(2\pi)^d}\langle u_n(\boldsymbol{k}_-)|\hat{s}_a|u_m(\boldsymbol{k}_+)\rangle\langle u_m(\boldsymbol{k}_+)|\hat{v}^j(\boldsymbol{k};\boldsymbol{Q})|u_n(\boldsymbol{k}_-)\rangle\frac{f(\epsilon_n(\boldsymbol{k}_-))-f(\epsilon_m(\boldsymbol{k}_+))}{\hbar\Omega+\epsilon_n(\boldsymbol{k}_-)-\epsilon_m(\boldsymbol{k}_+)+i\eta}\\=&\chi_{\hat{s}_a\hat{j}^j}(0,\boldsymbol{Q})+(i\Omega)\alpha^{\mathrm{R}}_{\hat{s}_a\hat{j}^j}(\Omega,\boldsymbol{Q}).\end{aligned} \tag{13}$$

We only have to expand the first term up to the first order with respect to $\boldsymbol{Q}$. The intraband $n=m$ and interband $n\neq m$ contributions are

$$\begin{aligned}\chi^{(\mathrm{I})}_{\hat{s}_a\hat{j}^j}(0,\boldsymbol{Q})=&-q\sum_n\int\frac{d^dk}{(2\pi)^d}\langle u_n(\boldsymbol{k}_-)|\hat{s}_a|u_n(\boldsymbol{k}_+)\rangle\langle u_n(\boldsymbol{k}_+)|\hat{v}^j(\boldsymbol{k};\boldsymbol{Q})|u_n(\boldsymbol{k}_-)\rangle\frac{f(\epsilon_n(\boldsymbol{k}_-))-f(\epsilon_n(\boldsymbol{k}_+))}{\epsilon_n(\boldsymbol{k}_-)-\epsilon_n(\boldsymbol{k}_+)}\\=&-q\sum_n\int\frac{d^dk}{(2\pi)^d}\langle u_n|\hat{s}_a|u_n\rangle\langle u_n|\hat{v}^j|u_n\rangle f'(\epsilon_n)+\frac{qQ_i}{2}\sum_n\int\frac{d^dk}{(2\pi)^d}\\&\times[(\langle\partial_{k_i}u_n|\hat{s}_a|u_n\rangle-\langle u_n|\hat{s}_a|\partial_{k_i}u_n\rangle)\langle u_n|\hat{v}^j|u_n\rangle-\langle u_n|\hat{s}_a|u_n\rangle(\langle\partial_{k_i}u_n|\hat{v}^j|u_n\rangle-\langle u_n|\hat{v}^j|\partial_{k_i}u_n\rangle)]f'(\epsilon_n)\\=&-q\sum_n\int\frac{d^dk}{(2\pi)^d}\langle u_n|\hat{s}_a|u_n\rangle\langle u_n|\hat{v}^j|u_n\rangle f'(\epsilon_n)\\&+\frac{qQ_i}{2}\sum_n\int\frac{d^dk}{(2\pi)^d}[(\langle\partial_{k_i}u_n|\hat{Q}_n\hat{s}_a|u_n\rangle-\text{c.c.})\langle u_n|\hat{v}^j|u_n\rangle-\langle u_n|\hat{s}_a|u_n\rangle(\langle\partial_{k_i}u_n|\hat{Q}_n\hat{v}^j|u_n\rangle-\text{c.c.})]f'(\epsilon_n)\\=&-\frac{q}{\hbar}\sum_n\int\frac{d^dk}{(2\pi)^d}s_{na}\partial_{k_j}\epsilon_nf'(\epsilon_n)+\frac{q(iQ_i)}{\hbar}\sum_n\int\frac{d^dk}{(2\pi)^d}({s_{na}}^i\partial_{k_j}\epsilon_n-s_{na}\epsilon^{ijk}m_{nk})f'(\epsilon_n),\end{aligned} \tag{14a}$$

$$\begin{aligned}\chi^{(\mathrm{II})}_{\hat{s}_a\hat{j}^j}(0,\boldsymbol{Q})=&-q\sum_{n\neq m}\int\frac{d^dk}{(2\pi)^d}\langle u_n(\boldsymbol{k}_-)|\hat{s}_a|u_m(\boldsymbol{k}_+)\rangle\langle u_m(\boldsymbol{k}_+)|\hat{v}^j(\boldsymbol{k};\boldsymbol{Q})|u_n(\boldsymbol{k}_-)\rangle\frac{f(\epsilon_n(\boldsymbol{k}_-))-f(\epsilon_m(\boldsymbol{k}_+))}{\epsilon_n(\boldsymbol{k}_-)-\epsilon_m(\boldsymbol{k}_+)}\\=&-q\sum_{n\neq m}\int\frac{d^dk}{(2\pi)^d}\langle u_n|\hat{s}_a|u_m\rangle\langle u_m|\hat{v}^j|u_n\rangle\frac{f(\epsilon_n)-f(\epsilon_m)}{\epsilon_n-\epsilon_m}+\frac{qQ_i}{2}\sum_{n\neq m}\int\frac{d^dk}{(2\pi)^d}\\&\times\Bigg\{[(\langle\partial_{k_i}u_n|\hat{s}_a|u_m\rangle-\langle u_n|\hat{s}_a|\partial_{k_i}u_m\rangle)\langle u_m|\hat{v}^j|u_n\rangle+\langle u_n|\hat{s}_a|u_m\rangle(\langle u_m|\hat{v}^j|\partial_{k_i}u_n\rangle-\langle\partial_{k_i}u_m|\hat{v}^j|u_n\rangle)]\\&\times\frac{f(\epsilon_n)-f(\epsilon_m)}{\epsilon_n-\epsilon_m}+\langle u_n|\hat{s}_a|u_m\rangle\langle u_m|\hat{v}^j|u_n\rangle\left[\frac{\partial_{k_i}\epsilon_nf'(\epsilon_n)+\partial_{k_i}\epsilon_mf'(\epsilon_m)}{\epsilon_n-\epsilon_m}-\frac{\partial_{k_i}(\epsilon_n+\epsilon_m)}{\epsilon_n-\epsilon_m}\frac{f(\epsilon_n)-f(\epsilon_m)}{\epsilon_n-\epsilon_m}\right]\Bigg\}\\=&-q\sum_{n\neq m}\int\frac{d^dk}{(2\pi)^d}\frac{\langle u_n|\hat{s}_a|u_m\rangle\langle u_m|\hat{v}^j|u_n\rangle+\text{c.c.}}{\epsilon_n-\epsilon_m}f(\epsilon_n)+\frac{qQ_i}{2}\sum_{n\neq m}\int\frac{d^dk}{(2\pi)^d}\\&\times\Bigg\{\frac{(\langle\partial_{k_i}u_n|\hat{s}_a|u_m\rangle-\langle u_n|\hat{s}_a|\partial_{k_i}u_m\rangle)\langle u_m|\hat{v}^j|u_n\rangle-\text{c.c.}+\langle u_n|\hat{s}_a|u_m\rangle(\langle u_m|\hat{v}^j|\partial_{k_i}u_n\rangle-\langle\partial_{k_i}u_m|\hat{v}^j|u_n\rangle)-\text{c.c.}}{\epsilon_n-\epsilon_m}\\&\times f(\epsilon_n)+\frac{\langle u_n|\hat{s}_a|u_m\rangle\langle u_m|\hat{v}^j|u_n\rangle-\text{c.c.}}{\epsilon_n-\epsilon_m}\left[\partial_{k_i}\epsilon_nf'(\epsilon_n)-\frac{\partial_{k_i}(\epsilon_n+\epsilon_m)}{\epsilon_n-\epsilon_m}f(\epsilon_n)\right]\Bigg\}\end{aligned}$$

$$
\begin{aligned}
=&-\frac{q}{\hbar}\sum_{n\neq m}\int\frac{d^dk}{(2\pi)^d}(\langle u_n|\hat{s}_a|u_m\rangle\langle u_m|\partial_{k_j}u_n\rangle+\text{c.c.})f(\epsilon_n)\\
&+\frac{qQ_i}{2\hbar}\sum_{n\neq m}\int\frac{d^dk}{(2\pi)^d}(\langle u_n|\hat{s}_a|u_m\rangle\langle u_m|\partial_{k_j}u_n\rangle-\text{c.c.})\partial_{k_i}\epsilon_n f'(\epsilon_n)+(\text{Fermi-sea terms})\\
=&-\frac{q}{\hbar}\sum_{n}\int\frac{d^dk}{(2\pi)^d}(\langle u_n|\hat{s}_a\hat{Q}_n|\partial_{k_j}u_n\rangle+\text{c.c.})f(\epsilon_n)\\
&+\frac{qQ_i}{2\hbar}\sum_{n}\int\frac{d^dk}{(2\pi)^d}(\langle u_n|\hat{s}_a\hat{Q}_n|\partial_{k_j}u_n\rangle-\text{c.c.})\partial_{k_i}\epsilon_n f'(\epsilon_n)+(\text{Fermi-sea terms})\\
=&-\frac{q}{\hbar}\sum_{n}\int\frac{d^dk}{(2\pi)^d}\partial_{k_j}s_{na}f(\epsilon_n)-\frac{q(iQ_i)}{\hbar}\sum_{n}\int\frac{d^dk}{(2\pi)^d}[s_{na}{}^j\partial_{k_i}\epsilon_n f'(\epsilon_n)+\epsilon^{ijk}b_{nak}f(\epsilon_n)].
\end{aligned}
\tag{14b}
$$

We can evaluate the Fermi-sea terms in Eq. (14b) by inserting $|u_l\rangle\langle u_l|$ as

$$
\begin{aligned}
&\frac{i\hbar}{2}\sum_{m(\neq n)}\frac{(\langle\partial_{k_i}u_n|\hat{s}_a|u_m\rangle-\langle u_n|\hat{s}_a|\partial_{k_i}u_m\rangle)\langle u_m|\hat{v}^j|u_n\rangle-\text{c.c.}+\langle u_n|\hat{s}_a|u_m\rangle(\langle u_m|\hat{v}^j|\partial_{k_i}u_n\rangle-\langle\partial_{k_i}u_m|\hat{v}^j|u_n\rangle)-\text{c.c.}}{\epsilon_n-\epsilon_m}\\
&-\frac{i\hbar}{2}\sum_{m(\neq n)}\frac{\langle u_n|\hat{s}_a|u_m\rangle\partial_{k_i}(\epsilon_n+\epsilon_m)\langle u_m|\hat{v}^j|u_n\rangle-\text{c.c.}}{(\epsilon_n-\epsilon_m)^2}\\
=&\frac{i\hbar}{2}\sum_{l\neq m(\neq n)}\Bigg[\frac{\langle\partial_{k_i}u_n|u_l\rangle\langle u_l|\hat{s}_a|u_m\rangle\langle u_m|\hat{v}^j|u_n\rangle-\text{c.c.}}{\epsilon_n-\epsilon_m}-\frac{\langle u_n|\hat{s}_a|u_l\rangle\langle u_l|\partial_{k_i}u_m\rangle\langle u_m|\hat{v}^j|u_n\rangle-\text{c.c.}}{\epsilon_n-\epsilon_m}\\
&+\frac{\langle u_n|\hat{s}_a|u_m\rangle\langle u_m|\hat{v}^j|u_l\rangle\langle u_l|\partial_{k_i}u_n\rangle-\text{c.c.}}{\epsilon_n-\epsilon_m}-\frac{\langle u_n|\hat{s}_a|u_m\rangle\langle\partial_{k_i}u_m|u_l\rangle\langle u_l|\hat{v}^j|u_n\rangle-\text{c.c.}}{\epsilon_n-\epsilon_m}\Bigg]\\
&+\frac{i\hbar}{2}\sum_{m(\neq n)}\Bigg[\frac{\langle\partial_{k_i}u_n|u_n\rangle\langle u_n|\hat{s}_a|u_m\rangle\langle u_m|\hat{v}^j|u_n\rangle-\text{c.c.}}{\epsilon_n-\epsilon_m}-\frac{\langle u_n|\hat{s}_a|u_n\rangle\langle u_n|\partial_{k_i}u_m\rangle\langle u_m|\hat{v}^j|u_n\rangle-\text{c.c.}}{\epsilon_n-\epsilon_m}\\
&+\frac{\langle u_n|\hat{s}_a|u_m\rangle\langle u_m|\hat{v}^j|u_n\rangle\langle u_n|\partial_{k_i}u_n\rangle-\text{c.c.}}{\epsilon_n-\epsilon_m}-\frac{\langle u_n|\hat{s}_a|u_m\rangle\langle\partial_{k_i}u_m|u_n\rangle\langle u_n|\hat{v}^j|u_n\rangle-\text{c.c.}}{\epsilon_n-\epsilon_m}\\
&+\frac{\langle\partial_{k_i}u_n|u_m\rangle\langle u_m|\hat{s}_a|u_m\rangle\langle u_m|\hat{v}^j|u_n\rangle-\text{c.c.}}{\epsilon_n-\epsilon_m}-\frac{\langle u_n|\hat{s}_a|u_m\rangle\langle u_m|\partial_{k_i}u_m\rangle\langle u_m|\hat{v}^j|u_n\rangle-\text{c.c.}}{\epsilon_n-\epsilon_m}\\
&+\frac{\langle u_n|\hat{s}_a|u_m\rangle\langle u_m|\hat{v}^j|u_m\rangle\langle u_m|\partial_{k_i}u_n\rangle-\text{c.c.}}{\epsilon_n-\epsilon_m}-\frac{\langle u_n|\hat{s}_a|u_m\rangle\langle\partial_{k_i}u_m|u_m\rangle\langle u_m|\hat{v}^j|u_n\rangle-\text{c.c.}}{\epsilon_n-\epsilon_m}\\
&-\frac{\langle u_n|\hat{s}_a|u_m\rangle\partial_{k_i}(\epsilon_n+\epsilon_m)\langle u_m|\hat{v}^j|u_n\rangle-\text{c.c.}}{(\epsilon_n-\epsilon_m)^2}\Bigg]\\
=&\frac{i\hbar^2}{2}\sum_{l\neq m(\neq n)}\Bigg[\frac{\langle u_n|\hat{v}^i|u_l\rangle\langle u_l|\hat{s}_a|u_m\rangle\langle u_m|\hat{v}^j|u_n\rangle-\text{c.c.}}{(\epsilon_n-\epsilon_m)(\epsilon_n-\epsilon_l)}-\frac{\langle u_n|\hat{s}_a|u_l\rangle\langle u_l|\hat{v}^i|u_m\rangle\langle u_m|\hat{v}^j|u_n\rangle-\text{c.c.}}{(\epsilon_n-\epsilon_m)(\epsilon_m-\epsilon_l)}\\
&+\frac{\langle u_n|\hat{s}_a|u_m\rangle\langle u_m|\hat{v}^j|u_l\rangle\langle u_l|\hat{v}^i|u_n\rangle-\text{c.c.}}{(\epsilon_n-\epsilon_m)(\epsilon_n-\epsilon_l)}-\frac{\langle u_n|\hat{s}_a|u_m\rangle\langle u_m|\hat{v}^i|u_l\rangle\langle u_l|\hat{v}^j|u_n\rangle-\text{c.c.}}{(\epsilon_n-\epsilon_m)(\epsilon_m-\epsilon_l)}\Bigg]\\
&+\frac{i\hbar^2}{2}\sum_{m(\neq n)}\Bigg[\frac{\langle u_n|\hat{s}_a|u_n\rangle\langle u_n|\hat{v}^i|u_m\rangle\langle u_m|\hat{v}^j|u_n\rangle-\text{c.c.}}{(\epsilon_n-\epsilon_m)^2}+\frac{\langle u_n|\hat{s}_a|u_m\rangle\langle u_m|\hat{v}^i|u_n\rangle\langle u_n|\hat{v}^j|u_n\rangle-\text{c.c.}}{(\epsilon_n-\epsilon_m)^2}\\
&+\frac{\langle u_n|\hat{v}^i|u_m\rangle\langle u_m|\hat{s}_a|u_m\rangle\langle u_m|\hat{v}^j|u_n\rangle-\text{c.c.}}{(\epsilon_n-\epsilon_m)^2}+\frac{\langle u_n|\hat{s}_a|u_m\rangle\langle u_m|\hat{v}^j|u_m\rangle\langle u_m|\hat{v}^i|u_n\rangle-\text{c.c.}}{(\epsilon_n-\epsilon_m)^2}\\
&-\frac{\langle u_n|\hat{s}_a|u_m\rangle(\langle u_n|\hat{v}^i|u_n\rangle+\langle u_m|\hat{v}^i|u_m\rangle)\langle u_m|\hat{v}^j|u_n\rangle-\text{c.c.}}{(\epsilon_n-\epsilon_m)^2}\Bigg]\\
=&\frac{i\hbar^2}{2}\sum_{l\neq m(\neq n)}\Bigg[\frac{\langle u_n|\hat{v}^i|u_m\rangle\langle u_m|\hat{s}_a|u_l\rangle\langle u_l|\hat{v}^j|u_n\rangle-\text{c.c.}}{(\epsilon_n-\epsilon_m)(\epsilon_n-\epsilon_l)}-\frac{\langle u_n|\hat{s}_a|u_m\rangle[\langle u_m|\hat{v}^i|u_l\rangle\langle u_l|\hat{v}^j|u_n\rangle-(i\leftrightarrow j)]-\text{c.c.}}{(\epsilon_n-\epsilon_m)(\epsilon_n-\epsilon_l)}\Bigg]\\
&+\frac{i\hbar^2}{2}\sum_{m(\neq n)}\Bigg\{\frac{\langle u_n|\hat{v}^i|u_m\rangle(\langle u_n|\hat{s}_a|u_n\rangle+\langle u_m|\hat{s}_a|u_m\rangle)\langle u_m|\hat{v}^j|u_n\rangle-\text{c.c.}}{(\epsilon_n-\epsilon_m)^2}
\end{aligned}
$$

$$
\begin{aligned}
&-\frac{\langle u_n|\hat{s}_a|u_m\rangle[(\langle u_n|\hat{v}^i|u_n\rangle+\langle u_m|\hat{v}^i|u_m\rangle)\langle u_m|\hat{v}^j|u_n\rangle-(i\leftrightarrow j)]-\text{c.c.}}{(\epsilon_n-\epsilon_m)^2}\Bigg\}\\
=&\frac{i\hbar^2}{2}\sum_{l,m(\neq n)}\Bigg[\frac{\langle u_n|\hat{v}^i|u_m\rangle\langle u_m|(\langle u_n|\hat{s}_a|u_n\rangle+\hat{s}_a)|u_l\rangle\langle u_l|\hat{v}^j|u_n\rangle-\text{c.c.}}{(\epsilon_n-\epsilon_m)(\epsilon_n-\epsilon_l)}\\
&-\frac{\langle u_n|\hat{s}_a|u_m\rangle[\langle u_m|(\langle u_n|\hat{v}^i|u_n\rangle+\hat{v}^i)|u_l\rangle\langle u_l|\hat{v}^j|u_n\rangle-(i\leftrightarrow j)]-\text{c.c.}}{(\epsilon_n-\epsilon_m)(\epsilon_n-\epsilon_l)}\Bigg]\\
=&\frac{i}{2}\sum_{l,m(\neq n)}[\langle\partial_{k_i}u_n|u_m\rangle\langle u_m|(s_{na}+\hat{s}_a)|u_l\rangle\langle u_l|\partial_{k_j}u_n\rangle-\text{c.c.}]\\
&-\frac{i}{2}\sum_{l,m(\neq n)}\frac{\langle u_n|\hat{s}_a|u_m\rangle[\langle u_m|(\partial_{k_i}\epsilon_n+\hbar\hat{v}^i)|u_l\rangle\langle u_l|\partial_{k_j}u_n\rangle-(i\leftrightarrow j)]-\text{c.c.}}{\epsilon_n-\epsilon_m}\\
=&\epsilon^{ijk}b_{nak}.
\end{aligned}
\tag{15}
$$

The first term of the Fermi-surface term (14a) is canceled by that of the Fermi-sea term (14b), and the second terms lead to the antisymmetry over $i$ and $j$. Finally, we arrive at the spin-orbit magnetic susceptibility,

$$
\chi^{\text{so}}_{ak}=-\frac{q}{\hbar}\sum_n\int\frac{d^dk}{(2\pi)^d}[(-\epsilon_{ijk}s_{na}{}^i\partial_{k_j}\epsilon_n+s_{na}m_{nk})f'(\epsilon_n)+b_{nak}f(\epsilon_n)].
\tag{16}
$$

## Spin accumulation

Next, we evaluate the second term in Eq. (13),

$$
\begin{aligned}
\alpha^{\text{R}}_{\hat{s}_a\hat{j}^j}(\Omega,\boldsymbol{Q})=&[\chi^{\text{R}}_{\hat{s}_a\hat{j}^j}(\Omega,\boldsymbol{Q})-\chi_{\hat{s}_a\hat{j}^j}(0,\boldsymbol{Q})]/(i\Omega)\\
=&-i\hbar q\sum_{nm}\int\frac{d^dk}{(2\pi)^d}\langle u_n(\boldsymbol{k}_-)|\hat{s}_a|u_m(\boldsymbol{k}_+)\rangle\langle u_m(\boldsymbol{k}_+)|\hat{v}^j(\boldsymbol{k};\boldsymbol{Q})|u_n(\boldsymbol{k}_-)\rangle\\
&\times\frac{f(\epsilon_n(\boldsymbol{k}_-))-f(\epsilon_m(\boldsymbol{k}_+))}{[\hbar\Omega+\epsilon_n(\boldsymbol{k}_-)-\epsilon_m(\boldsymbol{k}_+)+i\eta][\epsilon_n(\boldsymbol{k}_-)-\epsilon_m(\boldsymbol{k}_+)]},
\end{aligned}
\tag{17}
$$

up to the first order with respect to $\boldsymbol{Q}$ with keeping $\Omega$ nonzero. When the system has the time-reversal symmetry, we only have to calculate the intraband $n=m$ contribution,

$$
\begin{aligned}
\alpha^{\text{R(I)}}_{\hat{s}_a\hat{j}^j}(\Omega,\boldsymbol{Q})=&-i\hbar q\sum_n\int\frac{d^dk}{(2\pi)^d}\langle u_n(\boldsymbol{k}_-)|\hat{s}_a|u_n(\boldsymbol{k}_+)\rangle\langle u_n(\boldsymbol{k}_+)|\hat{v}^j(\boldsymbol{k};\boldsymbol{Q})|u_n(\boldsymbol{k}_-)\rangle\\
&\times\frac{f(\epsilon_n(\boldsymbol{k}_-))-f(\epsilon_n(\boldsymbol{k}_+))}{[\hbar\Omega+\epsilon_n(\boldsymbol{k}_-)-\epsilon_n(\boldsymbol{k}_+)+i\eta][\epsilon_n(\boldsymbol{k}_-)-\epsilon_n(\boldsymbol{k}_+)]}\\
=&-\frac{i\hbar q}{\hbar\Omega+i\eta}\sum_n\int\frac{d^dk}{(2\pi)^d}\langle u_n|\hat{s}_a|u_n\rangle\langle u_n|\hat{v}^j|u_n\rangle f'(\epsilon_n)\\
&-\frac{i\hbar qQ_i}{(\hbar\Omega+i\eta)^2}\sum_n\int\frac{d^dk}{(2\pi)^d}\langle u_n|\hat{s}_a|u_n\rangle\langle u_n|\hat{v}^j|u_n\rangle\partial_{k_i}\epsilon_nf'(\epsilon_n)\\
&+\frac{i\hbar qQ_i}{2(\hbar\Omega+i\eta)}\sum_n\int\frac{d^dk}{(2\pi)^d}\\
&\times[(\langle\partial_{k_i}u_n|\hat{s}_a|u_n\rangle-\langle u_n|\hat{s}_a|\partial_{k_i}u_n\rangle)\langle u_n|\hat{v}^j|u_n\rangle-\langle u_n|\hat{s}_a|u_n\rangle(\langle\partial_{k_i}u_n|\hat{v}^j|u_n\rangle-\langle u_n|\hat{v}^j|\partial_{k_i}u_n\rangle)]f'(\epsilon_n)\\
=&-\frac{iq}{\hbar\Omega+i\eta}\sum_n\int\frac{d^dk}{(2\pi)^d}s_{na}\partial_{k_j}\epsilon_nf'(\epsilon_n)-\frac{q(iQ_i)}{(\hbar\Omega+i\eta)^2}\sum_n\int\frac{d^dk}{(2\pi)^d}s_{na}\partial_{k_i}\epsilon_n\partial_{k_j}\epsilon_nf'(\epsilon_n)\\
&+\frac{iq(iQ_i)}{\hbar\Omega+i\eta}\sum_n\int\frac{d^dk}{(2\pi)^d}(s_{na}{}^i\partial_{k_j}\epsilon_n-s_{na}\epsilon^{ijk}m_{nk})f'(\epsilon_n).
\end{aligned}
\tag{18}
$$

Thus, the spin density induced by electromagnetic fields is summarized as

$$\langle \Delta\hat{s}_a\rangle(\Omega,\boldsymbol{Q}) =\frac{i\hbar}{\hbar\Omega+i\eta}{\alpha_a}^{j}E_j(\Omega,\boldsymbol{Q})+\left[\frac{\hbar^2}{(\hbar\Omega+i\eta)^2}{\gamma_a}^{ij(\mathrm{I})}-\frac{i\hbar}{\hbar\Omega+i\eta}{\gamma_a}^{ij(\mathrm{II})}\right](iQ_i)E_j(\Omega,\boldsymbol{Q})+\chi^{\mathrm{so}}_{ak}B^k(\Omega,\boldsymbol{Q}), \tag{19a}$$

$${\alpha_a}^{j} =-\frac{q}{\hbar}\sum_n\int\frac{d^dk}{(2\pi)^d}s_{na}\partial_{k_j}\epsilon_n f'(\epsilon_n), \tag{19b}$$

$${\gamma_a}^{ij(\mathrm{I})} =-\frac{q}{\hbar^2}\sum_n\int\frac{d^dk}{(2\pi)^d}s_{na}\partial_{k_i}\epsilon_n\partial_{k_j}\epsilon_n f'(\epsilon_n), \tag{19c}$$

$${\gamma_a}^{ij(\mathrm{II})} =-\frac{q}{\hbar}\sum_n\int\frac{d^dk}{(2\pi)^d}({s_{na}}^{i}\partial_{k_j}\epsilon_n - s_{na}\epsilon^{ijk}m_{nk})f'(\epsilon_n). \tag{19d}$$

## TWO-BAND MODELS

### Generic formulas for two-band models

Any two-band model can be represented as $\hat{\mathcal{H}}(\boldsymbol{k}) = h^0(\boldsymbol{k})+\boldsymbol{h}(\boldsymbol{k})\cdot\boldsymbol{\sigma}$. Below, the argument of $\boldsymbol{k}$ is omitted for simplicity. Now we assume that the Pauli matrix $\boldsymbol{\sigma}$ corresponds to the spin operator $\hat{\boldsymbol{s}}=(\hbar/2)\boldsymbol{\sigma}$.

First, we write down two-band formulas for the quantities defined above as well as the Berry curvature. The eigenvalues of the Hamiltonian are $\epsilon_\sigma = h^0+\sigma|\boldsymbol{h}|$, and the corresponding eigenstates are $|u_\sigma\rangle = [\sigma+\hat{h}^z, \hat{h}^x+i\hat{h}^y]^{\mathrm{t}}/\sqrt{2(1+\sigma\hat{h}^z)}$ with $\hat{\boldsymbol{h}}=\boldsymbol{h}/|\boldsymbol{h}|$. Using

$$\langle u_{-\sigma}|\partial_{k_j}u_\sigma\rangle =\frac{1}{2\sqrt{1-(\hat{h}^z)^2}}[-\sigma\partial_{k_j}\hat{h}^z+i(\hat{h}^x\partial_{k_j}\hat{h}^y-\hat{h}^y\partial_{k_j}\hat{h}^x)], \tag{20a}$$

$$\langle u_{-\sigma}|\boldsymbol{\sigma}|u_\sigma\rangle =\frac{1}{\sqrt{1-(\hat{h}^z)^2}}\begin{bmatrix}\hat{h}^x\hat{h}^z-i\sigma\hat{h}^y\\ \hat{h}^y\hat{h}^z+i\sigma\hat{h}^x\\ -[1-(\hat{h}^z)^2]\end{bmatrix}, \tag{20b}$$

$$\langle u_{-\sigma}|\frac{1}{2}\{\boldsymbol{\sigma},\hbar\hat{v}^i\}|u_\sigma\rangle =\langle u_{-\sigma}|(\partial_{k_i}\boldsymbol{h}+\partial_{k_i}h^0\boldsymbol{\sigma})|u_\sigma\rangle = \partial_{k_i}h^0\langle u_{-\sigma}|\boldsymbol{\sigma}|u_\sigma\rangle, \tag{20c}$$

we obtain

$$\begin{aligned}\epsilon^{ijk}b_{\sigma k} =& -2\,\mathrm{Im}[\langle\partial_{k_i}u_\sigma|u_{-\sigma}\rangle\langle u_{-\sigma}|\partial_{k_j}u_\sigma\rangle]\\
=&-\frac{\sigma}{2[1-(\hat{h}^z)^2]}[\hat{h}^x(\partial_{k_i}\hat{h}^y\partial_{k_j}\hat{h}^z-\partial_{k_i}\hat{h}^z\partial_{k_j}\hat{h}^y)+\hat{h}^y(\partial_{k_i}\hat{h}^z\partial_{k_j}\hat{h}^x-\partial_{k_i}\hat{h}^x\partial_{k_j}\hat{h}^z)]\\
=&-\frac{\sigma}{2}[\hat{h}^x(\partial_{k_i}\hat{h}^y\partial_{k_j}\hat{h}^z-\partial_{k_i}\hat{h}^z\partial_{k_j}\hat{h}^y)+\hat{h}^y(\partial_{k_i}\hat{h}^z\partial_{k_j}\hat{h}^x-\partial_{k_i}\hat{h}^x\partial_{k_j}\hat{h}^z)]\\
&-\frac{\sigma}{2[1-(\hat{h}^z)^2]}\hat{h}^z[(\hat{h}^x\partial_{k_i}\hat{h}^y-\hat{h}^y\partial_{k_i}\hat{h}^x)\hat{h}^z\partial_{k_j}\hat{h}^z-\hat{h}^z\partial_{k_i}\hat{h}^z(\hat{h}^x\partial_{k_j}\hat{h}^y-\hat{h}^y\partial_{k_j}\hat{h}^x)]\\
=&-\frac{\sigma}{2}[\hat{h}^x(\partial_{k_i}\hat{h}^y\partial_{k_j}\hat{h}^z-\partial_{k_i}\hat{h}^z\partial_{k_j}\hat{h}^y)+\hat{h}^y(\partial_{k_i}\hat{h}^z\partial_{k_j}\hat{h}^x-\partial_{k_i}\hat{h}^x\partial_{k_j}\hat{h}^z)]\\
&-\frac{\sigma}{2[1-(\hat{h}^z)^2]}\hat{h}^z[-(\hat{h}^x\partial_{k_i}\hat{h}^y-\hat{h}^y\partial_{k_i}\hat{h}^x)(\hat{h}^x\partial_{k_j}\hat{h}^x+\hat{h}^y\partial_{k_j}\hat{h}^y)+(\hat{h}^x\partial_{k_i}\hat{h}^x+\hat{h}^y\partial_{k_i}\hat{h}^y)(\hat{h}^x\partial_{k_j}\hat{h}^y-\hat{h}^y\partial_{k_j}\hat{h}^x)]\\
=&-\frac{\sigma}{2}[\hat{h}^x(\partial_{k_i}\hat{h}^y\partial_{k_j}\hat{h}^z-\partial_{k_i}\hat{h}^z\partial_{k_j}\hat{h}^y)+\hat{h}^y(\partial_{k_i}\hat{h}^z\partial_{k_j}\hat{h}^x-\partial_{k_i}\hat{h}^x\partial_{k_j}\hat{h}^z)]\\
&-\frac{\sigma}{2[1-(\hat{h}^z)^2]}\hat{h}^z[(\hat{h}^x)^2+(\hat{h}^y)^2](\partial_{k_i}\hat{h}^x\partial_{k_j}\hat{h}^y-\partial_{k_i}\hat{h}^y\partial_{k_j}\hat{h}^x)\\
=&-\frac{\sigma}{2}\hat{\boldsymbol{h}}\cdot\partial_{k_i}\hat{\boldsymbol{h}}\times\partial_{k_j}\hat{\boldsymbol{h}},\end{aligned} \tag{21a}$$

$$\epsilon^{ijk}m_{\sigma k} =-\sigma|\boldsymbol{h}|\epsilon^{ijk}b_{\sigma k}, \tag{21b}$$

$${s_{\sigma a}}^{i} =\frac{\hbar}{2}\,\mathrm{Im}[\partial_{k_i}u_\sigma|u_{-\sigma}\rangle\langle u_{-\sigma}|\sigma_a|u_\sigma\rangle]$$

$$
\begin{aligned}
=&\frac{\hbar}{2}\frac{1}{2[1-(\hat{h}^z)^2]}\begin{bmatrix}\hat{h}^y\partial_{k_i}\hat{h}^z-(\hat{h}^x)^2\hat{h}^z\partial_{k_i}\hat{h}^y+\hat{h}^y\hat{h}^z\hat{h}^x\partial_{k_i}\hat{h}^x\\(\hat{h}^y)^2\hat{h}^z\partial_{k_i}\hat{h}^x-\hat{h}^x\partial_{k_i}\hat{h}^z-\hat{h}^x\hat{h}^z\hat{h}^y\partial_{k_i}\hat{h}^y\\ [1-(\hat{h}^z)^2](\hat{h}^x\partial_{k_i}\hat{h}^y-\hat{h}^y\partial_{k_i}\hat{h}^x)\end{bmatrix}_a\\
=&\frac{\hbar}{2}\frac{1}{2[1-(\hat{h}^z)^2]}\begin{bmatrix}\hat{h}^y\partial_{k_i}\hat{h}^z-(\hat{h}^x)^2\hat{h}^z\partial_{k_i}\hat{h}^y-\hat{h}^y\hat{h}^z(\hat{h}^y\partial_{k_i}\hat{h}^y+\hat{h}^z\partial_{k_i}\hat{h}^z)\\(\hat{h}^y)^2\hat{h}^z\partial_{k_i}\hat{h}^x-\hat{h}^x\partial_{k_i}\hat{h}^z+\hat{h}^x\hat{h}^z(\hat{h}^x\partial_{k_i}\hat{h}^x+\hat{h}^z\partial_{k_i}\hat{h}^z)\\ [1-(\hat{h}^z)^2](\hat{h}^x\partial_{k_i}\hat{h}^y-\hat{h}^y\partial_{k_i}\hat{h}^x)\end{bmatrix}_a\\
=&\frac{\hbar}{2}\frac{1}{2[1-(\hat{h}^z)^2]}\begin{bmatrix}[1-(\hat{h}^z)^2]\hat{h}^y\partial_{k_i}\hat{h}^z-[(\hat{h}^x)^2+(\hat{h}^y)^2]\hat{h}^z\partial_{k_i}\hat{h}^y\\ [(\hat{h}^x)^2+(\hat{h}^y)^2]\hat{h}^z\partial_{k_i}\hat{h}^x-[1-(\hat{h}^z)^2]\hat{h}^x\partial_{k_i}\hat{h}^z\\ [1-(\hat{h}^z)^2](\hat{h}^x\partial_{k_i}\hat{h}^y-\hat{h}^y\partial_{k_i}\hat{h}^x)\end{bmatrix}_a\\
=&\frac{\hbar}{4}(\hat{\boldsymbol{h}}\times\partial_{k_i}\hat{\boldsymbol{h}})_a, \qquad (21c)\\
{b_{s\sigma a}}^{ij}=&\frac{\sigma\partial_{k_i}h^0}{|\boldsymbol{h}|}{s_{\sigma a}}^j, \qquad (21d)\\
\epsilon^{ijk}b_{\sigma ak}=&-\frac{\sigma\partial_{k_i}h^0}{|\boldsymbol{h}|}{s_{\sigma a}}^j-(i\leftrightarrow j). \qquad (21e)
\end{aligned}
$$

## Rashba model

The Rashba model is expressed as

$$\hat{\mathcal{H}}=\frac{\hbar^2k^2}{2m}+\hbar\alpha(k_y\sigma_x-k_x\sigma_y). \qquad (22)$$

Using the above formulas (21), we obtain ${s_{\sigma z}}^x=-(\hbar/4k)\sin\phi$, ${s_{\sigma z}}^y=(\hbar/4k)\cos\phi$, ${b_{s\sigma z}}^{xy}=(\sigma\hbar^2/4m\alpha k)\cos^2\phi$, and $b_{\sigma zz}=-\sigma\hbar^2/4m\alpha k$. Thus, the spin Hall conductivities of the conventional (5) and conserved spin currents (12), the spin-orbit magnetic susceptibility (16), and the spin accumulation (19d) are

$$
\begin{aligned}
{\sigma_{sz}}^{xy(\mathrm{II})}=&-\frac{q}{4}\sum_\sigma\sigma\int\frac{d^2k}{(2\pi)^2}\frac{\hbar\cos^2\phi}{m\alpha k}f(\epsilon_\sigma)\\
=&-\frac{q}{16\pi}\sum_\sigma\sigma\int_0^\infty dx f(\epsilon_\sigma(x)), \qquad (23a)\\
{\tilde{\sigma}_{sz}}^{xy(\mathrm{II})}=&-\frac{q}{4}\sum_\sigma\int\frac{d^2k}{(2\pi)^2}\left[\frac{\partial_k\epsilon_\sigma}{k}f'(\epsilon_\sigma)\cos^2\phi-\frac{\sigma\hbar}{m\alpha k}f(\epsilon_\sigma)\right]\\
=&-\frac{q}{16\pi}\sum_\sigma\int_0^\infty dx[\partial_x\epsilon_\sigma(x)f'(\epsilon_\sigma(x))-2\sigma f(\epsilon_\sigma(x))], \qquad (23b)\\
\chi^{\mathrm{so}}_{zz}=&-\frac{q}{4}\sum_\sigma\int\frac{d^2k}{(2\pi)^2}\left[\frac{\partial_k\epsilon_\sigma}{k}f'(\epsilon_\sigma)-\frac{\sigma\hbar}{m\alpha k}f(\epsilon_\sigma)\right]\\
=&-\frac{q}{8\pi}\sum_\sigma\int_0^\infty dx[\partial_x\epsilon_\sigma(x)f'(\epsilon_\sigma(x))-\sigma f(\epsilon_\sigma(x))], \qquad (23c)\\
{\gamma_z}^{xy(\mathrm{II})}=&\frac{q}{4}\sum_\sigma\int\frac{d^2k}{(2\pi)^2}\frac{\partial_k\epsilon_\sigma}{k}f'(\epsilon_\sigma)\sin^2\phi\\
=&\frac{q}{16\pi}\sum_\sigma\int_0^\infty dx\partial_x\epsilon_\sigma(x)f'(\epsilon_\sigma(x)). \qquad (23d)
\end{aligned}
$$

Here, we have introduced $x=\hbar k/m\alpha$ and $\epsilon_\sigma(x)=m\alpha^2(x^2/2+\sigma x)$. Note that the dimensionless Fermi wave numbers are $x_{\mathrm{F}\sigma}=-\sigma+\sqrt{1+2\mu/m\alpha^2}$ for $\mu>0$ while $x_{\mathrm{F}-}^{(\pm)}=1\pm\sqrt{1+2\mu/m\alpha^2}$ for $\mu<0$. At $T=0$, we obtain

$$
{\sigma_{sz}}^{xy(\mathrm{II})}=\frac{q}{8\pi}\begin{cases}1 & (\mu>0)\\ \sqrt{1+2\mu/m\alpha^2} & (\mu<0)\end{cases}, \qquad (24a)
$$

$$\tilde{\sigma}_{sz}{}^{xy(\mathrm{II})} = -\frac{q}{8\pi}\begin{cases}1 & (\mu>0)\\ 2\sqrt{1+2\mu/m\alpha^2} & (\mu<0)\end{cases}, \tag{24b}$$

$$\chi_{zz}^{\mathrm{so}} = -\frac{q}{4\pi}\begin{cases}0 & (\mu>0)\\ \sqrt{1+2\mu/m\alpha^2} & (\mu<0)\end{cases}, \tag{24c}$$

$$\gamma_z{}^{xy(\mathrm{II})} = -\frac{q}{8\pi}\begin{cases}1 & (\mu>0)\\ 0 & (\mu<0)\end{cases}, \tag{24d}$$

These results except for Eq. (24d) were already obtained [1, 3, 10].

## GREEN'S FUNCTIONS

### Green's functions

We consider $\delta$-function nonmagnetic disorder within the first-order Born approximation for the Rashba model (22). The bare retarded Green's function is expressed as

$$\hat{g}^{\mathrm{R}}(\epsilon,\boldsymbol{k}) = \frac{1}{\epsilon+i\eta-\hat{\mathcal{H}}(\boldsymbol{k})} = \frac{1}{2}[g_+^{\mathrm{R}}(\epsilon,\boldsymbol{k})+g_-^{\mathrm{R}}(\epsilon,\boldsymbol{k})] + \frac{1}{2}[g_+^{\mathrm{R}}(\epsilon,\boldsymbol{k})-g_-^{\mathrm{R}}(\epsilon,\boldsymbol{k})](\sigma_x\sin\phi-\sigma_y\cos\phi), \tag{25}$$

where $g_\sigma^{\mathrm{R}}(\epsilon,\boldsymbol{k}) = [\epsilon+i\eta-\epsilon_\sigma(\boldsymbol{k})]^{-1}$ is the diagonalized one. In the first-order Born approximation, the imaginary part of the self-energy is

$$\hat{\Gamma}(\epsilon) = -\operatorname{Im}\left[n_{\mathrm{i}}v_{\mathrm{i}}^2\int\frac{d^2k}{(2\pi)^2}\hat{g}^{\mathrm{R}}(\epsilon,\boldsymbol{k})\right] = \Gamma_0 d(\epsilon), \tag{26}$$

in which $\Gamma_0 = mn_{\mathrm{i}}v_{\mathrm{i}}^2/2\hbar^2$, and

$$d(\epsilon) = \frac{m\alpha^2}{2}\sum_\sigma\int_0^\infty dx x\frac{-1}{\pi}\operatorname{Im}[g_\sigma^{\mathrm{R}}(\epsilon,x)] = \begin{cases}1 & (\epsilon>0)\\ 1/\sqrt{1+2\epsilon/m\alpha^2} & (\epsilon<0)\end{cases}, \tag{27}$$

is the dimensionless density of states. The renormalized retarded Green's function is expressed as

$$\hat{G}^{\mathrm{R}}(\epsilon,\boldsymbol{k}) = \frac{1}{\epsilon+i\Gamma(\epsilon)-\hat{\mathcal{H}}(\boldsymbol{k})} = \frac{1}{2}[G_+^{\mathrm{R}}(\epsilon,\boldsymbol{k})+G_-^{\mathrm{R}}(\epsilon,\boldsymbol{k})] + \frac{1}{2}[G_+^{\mathrm{R}}(\epsilon,\boldsymbol{k})-G_-^{\mathrm{R}}(\epsilon,\boldsymbol{k})](\sigma_x\sin\phi-\sigma_y\cos\phi), \tag{28}$$

with $G_\sigma^{\mathrm{R}}(\epsilon,\boldsymbol{k}) = [\epsilon+i\Gamma(\epsilon)-\epsilon_\sigma(\boldsymbol{k})]^{-1}$ being the diagonalized one [11, 12].

### Spin-orbit magnetic susceptibility and spin accumulation

Let us calculate the spin-orbit magnetic susceptibility and spin accumulation. The spin response to a vector potential is expressed in terms of the Keldysh Green's function $\hat{G}(\epsilon,\boldsymbol{k})$ as

$$\begin{aligned}\langle\Delta\hat{s}_z\rangle(\Omega,\boldsymbol{Q}) =& iqA_y(\Omega,\boldsymbol{Q})\int\frac{d\epsilon}{2\pi}\int\frac{d^2k}{(2\pi)^2}\operatorname{tr}[\hat{s}_z\hat{G}(\epsilon_+,\boldsymbol{k}_+)\hat{v}^y(\boldsymbol{k};\boldsymbol{Q})\hat{G}(\epsilon_-,\boldsymbol{k}_-)]^<\\ =& iqA_y(\Omega,\boldsymbol{Q})\int\frac{d\epsilon}{2\pi}\int\frac{d^2k}{(2\pi)^2}\operatorname{tr}\{\hat{s}_z[\hat{G}^{\mathrm{A}}(\epsilon_+,\boldsymbol{k}_+)-\hat{G}^{\mathrm{R}}(\epsilon_+,\boldsymbol{k}_+)]\hat{v}^y(\boldsymbol{k};\boldsymbol{Q})\hat{G}^{\mathrm{A}}(\epsilon_-,\boldsymbol{k}_-)f(\epsilon_+)\\ &+\hat{s}_z\hat{G}^{\mathrm{R}}(\epsilon_+,\boldsymbol{k}_+)\hat{v}^y(\boldsymbol{k};\boldsymbol{Q})[\hat{G}^{\mathrm{A}}(\epsilon_-,\boldsymbol{k}_-)-\hat{G}^{\mathrm{R}}(\epsilon_-,\boldsymbol{k}_-)]f(\epsilon_-)\}\\ =& iqA_y(\Omega,\boldsymbol{Q})\int\frac{d\epsilon}{2\pi}\int\frac{d^2k}{(2\pi)^2}\operatorname{tr}\{-\hat{s}_z\hat{G}^{\mathrm{R}}(\epsilon_+,\boldsymbol{k}_+)\hat{v}^y(\boldsymbol{k};\boldsymbol{Q})\hat{G}^{\mathrm{A}}(\epsilon_-,\boldsymbol{k}_-)[f(\epsilon_+)-f(\epsilon_-)]\\ &+\hat{s}_z\hat{G}^{\mathrm{A}}(\epsilon_+,\boldsymbol{k}_+)\hat{v}^y(\boldsymbol{k};\boldsymbol{Q})\hat{G}^{\mathrm{A}}(\epsilon_-,\boldsymbol{k}_-)f(\epsilon_+)-\hat{s}_z\hat{G}^{\mathrm{R}}(\epsilon_+,\boldsymbol{k}_+)\hat{v}^y(\boldsymbol{k};\boldsymbol{Q})\hat{G}^{\mathrm{R}}(\epsilon_-,\boldsymbol{k}_-)f(\epsilon_-)\},\end{aligned} \tag{29}$$

with $\epsilon_\pm = \epsilon\pm\hbar\Omega/2$. Note that the lesser Green's function $G^<(\epsilon,\boldsymbol{k})$ satisfies

$$G^<(\epsilon,\boldsymbol{k}) = [G^{\mathrm{A}}(\epsilon,\boldsymbol{k})-G^{\mathrm{R}}(\epsilon,\boldsymbol{k})]f(\epsilon). \tag{30}$$

We expand Eq. (29) up to the first order with respect to $\Omega$ and $Q_x$ and obtain

$$\begin{aligned}\langle\Delta\hat{s}_z\rangle(\Omega,\boldsymbol{Q}) =&iqA_y(\Omega,\boldsymbol{Q})\int\frac{d\epsilon}{2\pi}\int\frac{d^2k}{(2\pi)^2}\,\mathrm{tr}\{-\hat{s}_z\hat{G}^{\mathrm{R}}(\epsilon_+,\boldsymbol{k})\hat{v}^y(\boldsymbol{k})\hat{G}^{\mathrm{A}}(\epsilon_-,\boldsymbol{k})[f(\epsilon_+)-f(\epsilon_-)]\\
&+\hat{s}_z\hat{G}^{\mathrm{A}}(\epsilon_+,\boldsymbol{k})\hat{v}^y(\boldsymbol{k})\hat{G}^{\mathrm{A}}(\epsilon_-,\boldsymbol{k})f(\epsilon_+)-\hat{s}_z\hat{G}^{\mathrm{R}}(\epsilon_+,\boldsymbol{k})\hat{v}^y(\boldsymbol{k})\hat{G}^{\mathrm{R}}(\epsilon_-,\boldsymbol{k})f(\epsilon_-)\}\\
&+\frac{i\hbar q}{2}Q_xA_y(\Omega,\boldsymbol{Q})\int\frac{d\epsilon}{2\pi}\int\frac{d^2k}{(2\pi)^2}\\
&\times\mathrm{tr}\{-\hat{s}_z\hat{G}^{\mathrm{R}}(\epsilon_+,\boldsymbol{k})[\hat{v}^x(\boldsymbol{k})\hat{G}^{\mathrm{R}}(\epsilon_+,\boldsymbol{k})\hat{v}^y(\boldsymbol{k})-\hat{v}^y(\boldsymbol{k})\hat{G}^{\mathrm{A}}(\epsilon_-,\boldsymbol{k})\hat{v}^x(\boldsymbol{k})]\hat{G}^{\mathrm{A}}(\epsilon_-,\boldsymbol{k})[f(\epsilon_+)-f(\epsilon_-)]\\
&+\hat{s}_z\hat{G}^{\mathrm{A}}(\epsilon_+,\boldsymbol{k})[\hat{v}^x(\boldsymbol{k})\hat{G}^{\mathrm{A}}(\epsilon_+,\boldsymbol{k})\hat{v}^y(\boldsymbol{k})-\hat{v}^y(\boldsymbol{k})\hat{G}^{\mathrm{A}}(\epsilon_-,\boldsymbol{k})\hat{v}^x(\boldsymbol{k})]\hat{G}^{\mathrm{A}}(\epsilon_-,\boldsymbol{k})f(\epsilon_+)\\
&-\hat{s}_z\hat{G}^{\mathrm{R}}(\epsilon_+,\boldsymbol{k})[\hat{v}^x(\boldsymbol{k})\hat{G}^{\mathrm{R}}(\epsilon_+,\boldsymbol{k})\hat{v}^y(\boldsymbol{k})-\hat{v}^y(\boldsymbol{k})\hat{G}^{\mathrm{R}}(\epsilon_-,\boldsymbol{k})\hat{v}^x(\boldsymbol{k})]\hat{G}^{\mathrm{R}}(\epsilon_-,\boldsymbol{k})f(\epsilon_-)\}\\
=&iqA_y(\Omega,\boldsymbol{Q})\int\frac{d\epsilon}{2\pi}f(\epsilon)\int\frac{d^2k}{(2\pi)^2}\,\mathrm{tr}[\hat{s}_z\hat{G}^{\mathrm{A}}\hat{v}^y\hat{G}^{\mathrm{A}}-(\mathrm{A}\to\mathrm{R})]\\
&+\frac{i\hbar q}{2}\Omega A_y(\Omega,\boldsymbol{Q})\int\frac{d\epsilon}{2\pi}f'(\epsilon)\int\frac{d^2k}{(2\pi)^2}\,\mathrm{tr}(-2\hat{s}_z\hat{G}^{\mathrm{R}}\hat{v}^y\hat{G}^{\mathrm{A}}+\hat{s}_z\hat{G}^{\mathrm{A}}\hat{v}^y\hat{G}^{\mathrm{A}}+\hat{s}_z\hat{G}^{\mathrm{R}}\hat{v}^y\hat{G}^{\mathrm{R}})\\
&+\frac{i\hbar q}{2}\Omega A_y(\Omega,\boldsymbol{Q})\int\frac{d\epsilon}{2\pi}f(\epsilon)\int\frac{d^2k}{(2\pi)^2}\,\mathrm{tr}[(\hat{s}_z\partial_\epsilon\hat{G}^{\mathrm{A}}\hat{v}^y\hat{G}^{\mathrm{A}}-\hat{s}_z\hat{G}^{\mathrm{A}}\hat{v}^y\partial_\epsilon\hat{G}^{\mathrm{A}})-(\mathrm{A}\to\mathrm{R})]\\
&+\frac{i\hbar q}{2}Q_xA_y(\Omega,\boldsymbol{Q})\int\frac{d\epsilon}{2\pi}f(\epsilon)\int\frac{d^2k}{(2\pi)^2}\,\mathrm{tr}[\hat{s}_z\hat{G}^{\mathrm{A}}(\hat{v}^x\hat{G}^{\mathrm{A}}\hat{v}^y-\hat{v}^y\hat{G}^{\mathrm{A}}\hat{v}^x)\hat{G}^{\mathrm{A}}-(\mathrm{A}\to\mathrm{R})]\\
&+\frac{i\hbar^2q}{4}\Omega Q_xA_y(\Omega,\boldsymbol{Q})\int\frac{d\epsilon}{2\pi}f'(\epsilon)\int\frac{d^2k}{(2\pi)^2}\,\mathrm{tr}[-2\hat{s}_z\hat{G}^{\mathrm{R}}(\hat{v}^x\hat{G}^{\mathrm{R}}\hat{v}^y-\hat{v}^y\hat{G}^{\mathrm{A}}\hat{v}^x)\hat{G}^{\mathrm{A}}\\
&+\hat{s}_z\hat{G}^{\mathrm{A}}(\hat{v}^x\hat{G}^{\mathrm{A}}\hat{v}^y-\hat{v}^y\hat{G}^{\mathrm{A}}\hat{v}^x)\hat{G}^{\mathrm{A}}+\hat{s}_z\hat{G}^{\mathrm{R}}(\hat{v}^x\hat{G}^{\mathrm{R}}\hat{v}^y-\hat{v}^y\hat{G}^{\mathrm{R}}\hat{v}^x)\hat{G}^{\mathrm{R}}]\\
&+\frac{i\hbar^2q}{4}\Omega Q_xA_y(\Omega,\boldsymbol{Q})\int\frac{d\epsilon}{2\pi}f(\epsilon)\int\frac{d^2k}{(2\pi)^2}\,\mathrm{tr}\{[\hat{s}_z\partial_\epsilon\hat{G}^{\mathrm{A}}(\hat{v}^x\hat{G}^{\mathrm{A}}\hat{v}^y-\hat{v}^y\hat{G}^{\mathrm{A}}\hat{v}^x)\hat{G}^{\mathrm{A}}\\
&+\hat{s}_z\hat{G}^{\mathrm{A}}(\hat{v}^x\partial_\epsilon\hat{G}^{\mathrm{A}}\hat{v}^y+\hat{v}^y\partial_\epsilon\hat{G}^{\mathrm{A}}\hat{v}^x)\hat{G}^{\mathrm{A}}-\hat{s}_z\hat{G}^{\mathrm{A}}(\hat{v}^x\hat{G}^{\mathrm{A}}\hat{v}^y-\hat{v}^y\hat{G}^{\mathrm{A}}\hat{v}^x)\partial_\epsilon\hat{G}^{\mathrm{A}}]-(\mathrm{A}\to\mathrm{R})\}.\end{aligned}\tag{31}$$

Here, we have omitted the arguments of $\epsilon$ and $\boldsymbol{k}$.

As expected from the $C_4$ symmetry, the zeroth-order terms with respect to $Q_x$ vanish;

$$\langle\Delta\hat{s}_z\rangle^{(0,0,\mathrm{II})}(\Omega,\boldsymbol{Q}) =iqA_y(\Omega,\boldsymbol{Q})\int\frac{d\epsilon}{2\pi}f(\epsilon)\int\frac{d^2k}{(2\pi)^2}\,\mathrm{tr}[\hat{s}_z\hat{G}^{\mathrm{A}}\hat{v}^y\hat{G}^{\mathrm{A}}-(\mathrm{A}\to\mathrm{R})]=0,\tag{32a}$$

$$\langle\Delta\hat{s}_z\rangle^{(1,0,\mathrm{I})}(\Omega,\boldsymbol{Q}) =\frac{i\hbar q}{2}\Omega A_y(\Omega,\boldsymbol{Q})\int\frac{d\epsilon}{2\pi}f'(\epsilon)\int\frac{d^2k}{(2\pi)^2}\,\mathrm{tr}(-2\hat{s}_z\hat{G}^{\mathrm{R}}\hat{V}^y\hat{G}^{\mathrm{A}}+\hat{s}_z\hat{G}^{\mathrm{A}}\hat{v}^y\hat{G}^{\mathrm{A}}+\hat{s}_z\hat{G}^{\mathrm{R}}\hat{v}^y\hat{G}^{\mathrm{R}})=0,\tag{32b}$$

$$\langle\Delta\hat{s}_z\rangle^{(1,0,\mathrm{II})}(\Omega,\boldsymbol{Q}) =\frac{i\hbar q}{2}\Omega A_y(\Omega,\boldsymbol{Q})\int\frac{d\epsilon}{2\pi}f(\epsilon)\int\frac{d^2k}{(2\pi)^2}\,\mathrm{tr}[(\hat{s}_z\partial_\epsilon\hat{G}^{\mathrm{A}}\hat{v}^y\hat{G}^{\mathrm{A}}-\hat{s}_z\hat{G}^{\mathrm{A}}\hat{v}^y\partial_\epsilon\hat{G}^{\mathrm{A}})-(\mathrm{A}\to\mathrm{R})]=0.\tag{32c}$$

In Eq. (32b), the bare vertex $\hat{v}^y(\boldsymbol{k})$ has been replaced by the renormalized vertex $\hat{V}^y(\epsilon,\boldsymbol{k})$. $\hat{V}^y(\epsilon,\boldsymbol{k})$ is obtained by solving

$$\hat{V}^y(\epsilon,\boldsymbol{k})=\hat{v}^y(\boldsymbol{k})+n_{\mathrm{i}}v_{\mathrm{i}}^2\int\frac{d^2k'}{(2\pi)^2}\hat{G}^{\mathrm{R}}(\epsilon,\boldsymbol{k}')\hat{V}^y(\epsilon,\boldsymbol{k}')\hat{G}^{\mathrm{A}}(\epsilon,\boldsymbol{k}').\tag{33}$$

For $\hat{v}^y(\boldsymbol{k})=\hbar k_y/m+\alpha\sigma_x$, we assume $\hat{V}^y(\epsilon,\boldsymbol{k})=\hbar k_y/m+\alpha V^{yx}(\epsilon)\sigma_x$ and obtain

$$\begin{aligned}V^{yx}(\epsilon)&=\left[1+\frac{n_{\mathrm{i}}v_{\mathrm{i}}^2}{4}\int_0^\infty\frac{kdk}{2\pi}(G_+^{\mathrm{A}}G_+^{\mathrm{R}}-G_-^{\mathrm{A}}G_-^{\mathrm{R}})\frac{\hbar k}{m\alpha}\right]\left[1-\frac{n_{\mathrm{i}}v_{\mathrm{i}}^2}{4}\int_0^\infty\frac{kdk}{2\pi}(G_+^{\mathrm{A}}+G_-^{\mathrm{A}}][G_+^{\mathrm{R}}+G_-^{\mathrm{R}})\right]^{-1}\\
&=\left\{1+\frac{\Gamma_0m\alpha^2}{4\Gamma(\epsilon)}\sum_\sigma\sigma\int_0^\infty dxx^2\frac{-1}{\pi}\,\mathrm{Im}[G_\sigma^{\mathrm{R}}(\epsilon,x)]\right\}\\
&\quad\times\left\{1-\frac{\Gamma_0m\alpha^2}{4\Gamma(\epsilon)}\sum_\sigma\int_0^\infty dxx\frac{-1}{\pi}\,\mathrm{Im}[G_\sigma^{\mathrm{R}}(\epsilon,x)]-\frac{\Gamma_0m\alpha^2}{4}\sum_\sigma\sigma\int_0^\infty dxx\frac{1}{\pi}\Re\left[\frac{G_\sigma^{\mathrm{R}}(\epsilon,x)}{m\alpha^2x-i\sigma\Gamma(\epsilon)}\right]\right\}^{-1}.\end{aligned}\tag{34}$$

The first-order terms are

$$
\begin{aligned}
\langle\Delta\hat{s}_z\rangle^{(0,1,\mathrm{II})}(\Omega,\boldsymbol{Q}) =&\frac{i\hbar q}{2}Q_xA_y(\Omega,\boldsymbol{Q})\int\frac{d\epsilon}{2\pi}f(\epsilon)\int\frac{d^2k}{(2\pi)^2}\,\mathrm{tr}[\hat{s}_z\hat{G}^{\mathrm{A}}(\hat{v}^x\hat{G}^{\mathrm{A}}\hat{v}^y-\hat{v}^y\hat{G}^{\mathrm{A}}\hat{v}^x)\hat{G}^{\mathrm{A}}-(\mathrm{A}\to\mathrm{R})]\\
=&\frac{i\hbar^2q\alpha}{m}Q_xA_y(\Omega,\boldsymbol{Q})\int\frac{d\epsilon}{2\pi}f(\epsilon)\int_0^\infty\frac{kdk}{2\pi}\,\mathrm{Im}[(\hbar k+m\alpha)(G^{\mathrm{R}}_+)^2G^{\mathrm{R}}_--(\hbar k-m\alpha)G^{\mathrm{R}}_+(G^{\mathrm{R}}_-)^2]\\
=&-\frac{q}{8\pi}B^z(\Omega,\boldsymbol{Q})\int d\epsilon f(\epsilon)\sum_\sigma\int_0^\infty dx\frac{-1}{\pi}\,\mathrm{Im}[\partial_xG^{\mathrm{R}}_\sigma(\epsilon,x)-\sigma G^{\mathrm{R}}_\sigma(\epsilon,x)],
\end{aligned}
\tag{35a}
$$

$$
\begin{aligned}
\langle\Delta\hat{s}_z\rangle^{(1,1,\mathrm{I})}(\Omega,\boldsymbol{Q}) =&\frac{i\hbar^2q}{4}\Omega Q_xA_y(\Omega,\boldsymbol{Q})\int\frac{d\epsilon}{2\pi}f'(\epsilon)\int\frac{d^2k}{(2\pi)^2}\,\mathrm{tr}[-2\hat{S}_z\hat{G}^{\mathrm{R}}(\hat{v}^x\hat{G}^{\mathrm{R}}\hat{V}^y-\hat{V}^y\hat{G}^{\mathrm{A}}\hat{v}^x)\hat{G}^{\mathrm{A}}\\
&+\hat{s}_z\hat{G}^{\mathrm{A}}(\hat{v}^x\hat{G}^{\mathrm{A}}\hat{v}^y-\hat{v}^y\hat{G}^{\mathrm{A}}\hat{v}^x)\hat{G}^{\mathrm{A}}+\hat{s}_z\hat{G}^{\mathrm{R}}(\hat{v}^x\hat{G}^{\mathrm{R}}\hat{v}^y-\hat{v}^y\hat{G}^{\mathrm{R}}\hat{v}^x)\hat{G}^{\mathrm{R}}]\\
=&\frac{\hbar^3q\alpha}{8m}\Omega Q_xA_y(\Omega,\boldsymbol{Q})\int\frac{d\epsilon}{2\pi}f'(\epsilon)\int_0^\infty\frac{kdk}{2\pi}\\
&\times\big([\hbar k+m\alpha V^{yx}(\epsilon)]S^z_z(\epsilon)G^{\mathrm{A}}_+G^{\mathrm{R}}_+(G^{\mathrm{A}}_-+G^{\mathrm{R}}_-)-[\hbar k-m\alpha V^{yx}(\epsilon)]S^z_z(\epsilon)G^{\mathrm{A}}_-G^{\mathrm{R}}_-(G^{\mathrm{A}}_++G^{\mathrm{R}}_+)\\
&+(\hbar k+m\alpha)\{V^{yx}(\epsilon)S^z_z(\epsilon)[(G^{\mathrm{A}}_+)^2G^{\mathrm{R}}_-+G^{\mathrm{A}}_-(G^{\mathrm{R}}_+)^2]-2[(G^{\mathrm{A}}_+)^2G^{\mathrm{A}}_-+(G^{\mathrm{R}}_+)^2G^{\mathrm{R}}_-]\}\\
&-(\hbar k-m\alpha)\{V^{yx}(\epsilon)S^z_z(\epsilon)[(G^{\mathrm{A}}_-)^2G^{\mathrm{R}}_++G^{\mathrm{A}}_+(G^{\mathrm{R}}_-)^2]-2[G^{\mathrm{A}}_+(G^{\mathrm{A}}_-)^2+G^{\mathrm{R}}_+(G^{\mathrm{R}}_-)^2]\}\big)\\
=&-\frac{\hbar q}{32\pi}(iQ_x)E_y(\Omega,\boldsymbol{Q})\int d\epsilon f'(\epsilon)\frac{S^z_z(\epsilon)}{\Gamma(\epsilon)}m\alpha^2\sum_\sigma\int_0^\infty dx[x+\sigma V^{yx}(\epsilon)]\frac{-1}{\pi}\,\mathrm{Im}[G^{\mathrm{R}}_\sigma(\epsilon,x)]\\
&-\frac{\hbar q}{32\pi}(iQ_x)E_y(\Omega,\boldsymbol{Q})\int d\epsilon f'(\epsilon)\sum_\sigma\int_0^\infty dx\frac{1}{\pi}\Re\left(\left[-2+\frac{m\alpha^2V^{yx}(\epsilon)S^z_z(\epsilon)x}{m\alpha^2x-i\sigma\Gamma(\epsilon)}\right]\partial_xG^{\mathrm{R}}_\sigma(\epsilon,x)\right.\\
&\left.+\sigma\left\{2-\frac{m\alpha^2S^z_z(\epsilon)x}{m\alpha^2x-i\sigma\Gamma(\epsilon)}-\frac{(m\alpha^2)^2V^{yx}(\epsilon)S^z_z(\epsilon)x^2}{[m\alpha^2x-i\sigma\Gamma(\epsilon)]^2}\right\}G^{\mathrm{R}}_\sigma(\epsilon,x)\right),
\end{aligned}
\tag{35b}
$$

$$
\begin{aligned}
\langle\Delta\hat{s}_z\rangle^{(1,1,\mathrm{II})}(\Omega,\boldsymbol{Q}) =&\frac{i\hbar^2q}{4}\Omega Q_xA_y(\Omega,\boldsymbol{Q})\int\frac{d\epsilon}{2\pi}f(\epsilon)\int\frac{d^2k}{(2\pi)^2}\,\mathrm{tr}\{[\hat{s}_z\partial_\epsilon\hat{G}^{\mathrm{A}}(\hat{v}^x\hat{G}^{\mathrm{A}}\hat{v}^y-\hat{v}^y\hat{G}^{\mathrm{A}}\hat{v}^x)\hat{G}^{\mathrm{A}}\\
&+\hat{s}_z\hat{G}^{\mathrm{A}}(\hat{v}^x\partial_\epsilon\hat{G}^{\mathrm{A}}\hat{v}^y+\hat{v}^y\partial_\epsilon\hat{G}^{\mathrm{A}}\hat{v}^x)\hat{G}^{\mathrm{A}}-\hat{s}_z\hat{G}^{\mathrm{A}}(\hat{v}^x\hat{G}^{\mathrm{A}}\hat{v}^y-\hat{v}^y\hat{G}^{\mathrm{A}}\hat{v}^x)\partial_\epsilon\hat{G}^{\mathrm{A}}]-(\mathrm{A}\to\mathrm{R})\}\\
=&0.
\end{aligned}
\tag{35c}
$$

In Eq. (35b), the bare vertices $\hat{v}^y(\boldsymbol{k})$ and $\hat{s}_z$ sandwiched by the $\hat{G}^{\mathrm{A}}(\epsilon,\boldsymbol{k})$ and $\hat{G}^{\mathrm{R}}(\epsilon,\boldsymbol{k})$ have been replaced by the renormalized vertices $\hat{V}^y(\epsilon,\boldsymbol{k})$ and $\hat{S}_z(\epsilon)$, respectively. $\hat{S}_z(\epsilon)$ is obtained by solving

$$
\hat{S}_z(\epsilon)=\hat{s}_z+n_{\mathrm{i}}v_{\mathrm{i}}^2\int\frac{d^2k'}{(2\pi)^2}\hat{G}^{\mathrm{A}}(\epsilon,\boldsymbol{k}')\hat{S}_z(\epsilon)\hat{G}^{\mathrm{R}}(\epsilon,\boldsymbol{k}'). \tag{36}
$$

For $\hat{s}_z=(\hbar/2)\sigma_z$, we assume $\hat{S}_z(\epsilon)=(\hbar/2)S^z_z(\epsilon)\sigma_z$ and obtain

$$
S^z_z(\epsilon)=\left[1-\frac{n_{\mathrm{i}}v_{\mathrm{i}}^2}{2}\int_0^\infty\frac{kdk}{2\pi}(G^{\mathrm{A}}_+G^{\mathrm{R}}_-+G^{\mathrm{A}}_-G^{\mathrm{R}}_+)\right]^{-1}=\left\{1-\frac{\Gamma_0m\alpha^2}{2}\sum_\sigma\sigma\int_0^\infty dxx\frac{1}{\pi}\Re\left[\frac{G^{\mathrm{R}}_\sigma(\epsilon,x)}{m\alpha^2x-i\sigma\Gamma(\epsilon)}\right]\right\}^{-1}. \tag{37}
$$

The Fermi-sea term (35c) vanishes owing to the time-reversal symmetry.

In the limit of $\Gamma_0\to+0$, we obtain

$$
\begin{aligned}
\langle\Delta\hat{s}_z\rangle^{(0,1,\mathrm{II})}(\Omega,\boldsymbol{Q}) =&-\frac{q}{8\pi}B^z(\Omega,\boldsymbol{Q})\int d\epsilon f(\epsilon)\sum_\sigma\int_0^\infty dx\frac{-1}{\pi}\,\mathrm{Im}[\partial_xg^{\mathrm{R}}_\sigma(\epsilon,x)-\sigma g^{\mathrm{R}}_\sigma(\epsilon,x)]\\
=&-\frac{q}{4\pi}B^z(\Omega,\boldsymbol{Q})\int d\epsilon f(\epsilon)\left[-\delta(\epsilon)+\frac{1}{m\alpha^2}\begin{cases}0 & (\epsilon>0)\\ 1/\sqrt{1+2\epsilon/m\alpha^2} & (\epsilon<0)\end{cases}\right],
\end{aligned}
\tag{38a}
$$

$$
\begin{aligned}
\langle\Delta\hat{s}_z\rangle^{(1,1,\mathrm{I})}(\Omega,\boldsymbol{Q}) =&-\frac{\hbar q}{32\pi}(iQ_x)E_y(\Omega,\boldsymbol{Q})\int d\epsilon f'(\epsilon)\frac{S^z_z(\epsilon)}{\Gamma(\epsilon)}m\alpha^2\sum_\sigma\int_0^\infty dx[x+\sigma V^{yx}(\epsilon)]\frac{-1}{\pi}\,\mathrm{Im}[g^{\mathrm{R}}_\sigma(\epsilon,x)]\\
=&-\frac{\hbar q}{16\pi}(iQ_x)E_y(\Omega,\boldsymbol{Q})\int d\epsilon f'(\epsilon)\frac{S^z_z(\epsilon)}{\Gamma(\epsilon)}\begin{cases}1 & (\epsilon>0)\\ [1-V^{yx}(\epsilon)]/\sqrt{1+2\epsilon/m\alpha^2} & (\epsilon<0)\end{cases},
\end{aligned}
\tag{38b}
$$

If we put $V^{yx}(\epsilon) = S^z_z(\epsilon) = 1$ to neglect the vertex corrections, we obtain

$$\chi^{\rm so}_{zz} = -\frac{q}{4\pi}\int d\epsilon f(\epsilon)\left[-\delta(\epsilon) + \frac{1}{m\alpha^2}\begin{cases}0 & (\epsilon > 0)\\ 1/\sqrt{1+2\epsilon/m\alpha^2} & (\epsilon < 0)\end{cases}\right], \tag{39a}$$

$$\langle \Delta\hat{s}_z\rangle^{(1,1,\mathrm{I})}(\Omega,\boldsymbol{Q}) = \frac{q}{8\pi}(iQ_x)E_y(\Omega,\boldsymbol{Q})\int d\epsilon f'(\epsilon)\frac{-\hbar}{2\Gamma(\epsilon)}\begin{cases}1 & (\epsilon > 0)\\ 0 & (\epsilon < 0)\end{cases}. \tag{39b}$$

When we take into account the vertex corrections (34) and (37), we reproduce [13]

$$\begin{aligned} V^{yx}(\epsilon) &= \left\{1 + \frac{\Gamma_0 m\alpha^2}{4\Gamma(\epsilon)}\sum_\sigma \sigma\int_0^\infty dx x^2\frac{-1}{\pi}\mathrm{Im}[g^{\rm R}_\sigma(\epsilon,x)]\right\}\left\{1 - \frac{\Gamma_0 m\alpha^2}{4\Gamma(\epsilon)}\sum_\sigma\int_0^\infty dx x\frac{-1}{\pi}\mathrm{Im}[g^{\rm R}_\sigma(\epsilon,x)]\right\}^{-1} \\ &= \begin{cases}0 & (\epsilon > 0)\\ -2\epsilon/m\alpha^2 & (\epsilon < 0)\end{cases}, \end{aligned} \tag{40}$$

and $S^z_z(\epsilon) = 1$ [14]. Hence, the correct spin accumulation is expressed as

$$\langle \Delta\hat{s}_z\rangle^{(1,1,\mathrm{I})}(\Omega,\boldsymbol{Q}) = \frac{q}{8\pi}(iQ_x)E_y(\Omega,\boldsymbol{Q})\int d\epsilon f'(\epsilon)\frac{-\hbar}{2\Gamma(\epsilon)}\begin{cases}1 & (\epsilon > 0)\\ \sqrt{1+2\epsilon/m\alpha^2} & (\epsilon < 0)\end{cases}. \tag{41}$$


[1] J. Sinova, D. Culcer, Q. Niu, N. A. Sinitsyn, T. Jungwirth, and A. H. MacDonald, Phys. Rev. Lett. **92**, 126603 (2004).
[2] J. Shi, P. Zhang, D. Xiao, and Q. Niu, Phys. Rev. Lett. **96**, 076604 (2006).
[3] P. Zhang, Z. Wang, J. Shi, D. Xiao, and Q. Niu, Phys. Rev. B **77**, 075304 (2008).
[4] G. Sundaram and Q. Niu, Phys. Rev. B **59**, 14915 (1999).
[5] D. Xiao, J. Shi, and Q. Niu, Phys. Rev. Lett. **95**, 137204 (2005).
[6] D. Xiao, J. Shi, and Q. Niu, Phys. Rev. Lett. **95**, 169903(E) (2005).
[7] Y. Gao, D. Vanderbilt, and D. Xiao, Phys. Rev. B **97**, 134423 (2018).
[8] A. Shitade, A. Daido, and Y. Yanase, Phys. Rev. B **99**, 024404 (2019).
[9] Y. Araki, D. Suenaga, K. Suzuki, and S. Yasui, Phys. Rev. Res. **3**, 023098 (2021).
[10] H. Suzuura and T. Ando, Phys. Rev. B **94**, 085303 (2016).
[11] A. Dyrdał, J. Barnaś, and V. K. Dugaev, Phys. Rev. B **94**, 035306 (2016).
[12] A. Dyrdał, J. Barnaś, and V. K. Dugaev, Phys. Rev. B **95**, 245302 (2017).
[13] J.-i. Inoue, G. E. W. Bauer, and L. W. Molenkamp, Phys. Rev. B **70**, 041303(R) (2004).
[14] V. M. Edelstein, Solid State Commun. **73**, 233 (1990).
